# Supplementary material for: Estimating the concentration parameter of a von Mises distribution: a systematic simulation benchmark
Source: arXiv:2111.09660 ancillary file (2021-11-18)
Supplement: Supplementary file 1 [file Supplement.pdf]

# Supplemental material for manuscript “Estimating the concentration parameter of a von Mises distribution: a systematic simulation benchmark”

G. Marrelec and A. Giron

## List of Tables

|    |                                                            |    |
|----|------------------------------------------------------------|----|
| 1  | Results for estimator <code>jML</code> . . . . .           | 2  |
| 2  | Results for estimator <code>mML</code> . . . . .           | 3  |
| 3  | Results for estimator <code>BF1</code> . . . . .           | 4  |
| 4  | Results for estimator <code>BF2</code> . . . . .           | 5  |
| 5  | Results for estimator <code>median1</code> . . . . .       | 6  |
| 6  | Results for estimator <code>median2</code> . . . . .       | 7  |
| 7  | Results for estimator <code>linear</code> . . . . .        | 8  |
| 8  | Results for estimator <code>MML-2</code> . . . . .         | 9  |
| 9  | Results for estimator <code>MML-3</code> . . . . .         | 10 |
| 10 | Results for estimator <code>BayesEst-2-km</code> . . . . . | 11 |
| 11 | Results for estimator <code>BayesEst-3-km</code> . . . . . | 12 |
| 12 | Results for estimator <code>BayesEst-3-xy</code> . . . . . | 13 |

## List of Figures

|   |                                                                                            |    |
|---|--------------------------------------------------------------------------------------------|----|
| 1 | Results for estimators <code>jML</code> and <code>mML</code> . . . . .                     | 14 |
| 2 | Results for estimators <code>BF1</code> and <code>BF2</code> . . . . .                     | 15 |
| 3 | Results for estimators <code>median1</code> and <code>median2</code> . . . . .             | 16 |
| 4 | Results for estimators <code>linear</code> and <code>MML-2</code> . . . . .                | 17 |
| 5 | Results for estimators <code>MML-3</code> and <code>BayesEst-2-km</code> . . . . .         | 18 |
| 6 | Results for estimators <code>BayesEst-3-km</code> and <code>BayesEst-3-xy</code> . . . . . | 19 |

| $\kappa$ | $N$  | Computation time |           | Error              |                    |        | 0.25    | 0.75   | min                   | max                |
|----------|------|------------------|-----------|--------------------|--------------------|--------|---------|--------|-----------------------|--------------------|
|          |      | mean             | std. dev. | mean               | std. dev.          | median |         |        |                       |                    |
| 0        | 2    | 26.8 ms          | 7.64 ms   | 269                | 2400               | 1.98   | 0.732   | 6.27   | $6.65 \times 10^{-6}$ | $5.52 \times 10^4$ |
|          | 4    | 27.2 ms          | 6.33 ms   | 1.42               | 2.93               | 0.946  | 0.574   | 1.47   | 0.0149                | 70.6               |
|          | 8    | 26.9 ms          | 6.38 ms   | 0.717              | 0.438              | 0.637  | 0.414   | 0.899  | 0.0271                | 3.46               |
|          | 16   | 26.6 ms          | 6.28 ms   | 0.455              | 0.257              | 0.42   | 0.268   | 0.594  | 0.0164                | 1.56               |
|          | 32   | 26.7 ms          | 6.39 ms   | 0.307              | 0.168              | 0.281  | 0.181   | 0.403  | 0.00462               | 0.947              |
|          | 64   | 26.5 ms          | 6.37 ms   | 0.224              | 0.113              | 0.21   | 0.142   | 0.292  | 0.00508               | 0.775              |
|          | 128  | 26.7 ms          | 6.32 ms   | 0.157              | 0.0802             | 0.149  | 0.097   | 0.205  | 0.00466               | 0.455              |
|          | 256  | 26.6 ms          | 6.49 ms   | 0.107              | 0.0578             | 0.0988 | 0.0649  | 0.142  | 0.00472               | 0.323              |
|          | 512  | 26.8 ms          | 6.42 ms   | 0.0757             | 0.0396             | 0.0718 | 0.0455  | 0.102  | 0.00287               | 0.206              |
|          | 1024 | 26.9 ms          | 6.23 ms   | 0.0553             | 0.0288             | 0.0517 | 0.034   | 0.0731 | 0.00107               | 0.165              |
|          | 2048 | 27.3 ms          | 6.5 ms    | 0.04               | 0.0204             | 0.0385 | 0.0243  | 0.0523 | 0.00189               | 0.115              |
|          | 4096 | 27.6 ms          | 6.6 ms    | 0.028              | 0.0143             | 0.0262 | 0.0171  | 0.0372 | $2.19 \times 10^{-4}$ | 0.0862             |
|          | 8192 | 27.2 ms          | 6.36 ms   | 0.0198             | 0.00996            | 0.0188 | 0.0121  | 0.0259 | $2.86 \times 10^{-4}$ | 0.0605             |
| 0.01     | 2    | 21.8 ms          | 4.2 ms    | 9260               | $2.61 \times 10^5$ | 2.03   | 0.771   | 6.4    | 0.00306               | $8.21 \times 10^6$ |
|          | 4    | 22 ms            | 3.92 ms   | 1.39               | 1.83               | 0.954  | 0.578   | 1.51   | 0.0136                | 24.2               |
|          | 8    | 22.2 ms          | 4.16 ms   | 0.701              | 0.433              | 0.619  | 0.387   | 0.942  | 0.0175                | 2.95               |
|          | 16   | 22.1 ms          | 4.08 ms   | 0.458              | 0.259              | 0.425  | 0.272   | 0.598  | 0.00134               | 1.74               |
|          | 32   | 22.2 ms          | 4.21 ms   | 0.311              | 0.171              | 0.29   | 0.182   | 0.419  | $1.57 \times 10^{-4}$ | 1.2                |
|          | 64   | 22.1 ms          | 3.93 ms   | 0.217              | 0.114              | 0.204  | 0.129   | 0.287  | 0.00626               | 0.614              |
|          | 128  | 22 ms            | 3.82 ms   | 0.153              | 0.088              | 0.143  | 0.0864  | 0.204  | $6.1 \times 10^{-4}$  | 0.519              |
|          | 256  | 22.1 ms          | 4.07 ms   | 0.103              | 0.0583             | 0.0944 | 0.0618  | 0.14   | $6.84 \times 10^{-5}$ | 0.306              |
|          | 512  | 22.1 ms          | 4.03 ms   | 0.0689             | 0.0403             | 0.0635 | 0.0392  | 0.0939 | $5.14 \times 10^{-4}$ | 0.207              |
|          | 1024 | 22.2 ms          | 3.97 ms   | 0.0465             | 0.0293             | 0.0434 | 0.0239  | 0.0644 | $4.26 \times 10^{-5}$ | 0.149              |
|          | 2048 | 22.3 ms          | 4.21 ms   | 0.0302             | 0.0205             | 0.0276 | 0.0137  | 0.0426 | $4.6 \times 10^{-5}$  | 0.113              |
|          | 4096 | 22.5 ms          | 4.34 ms   | 0.0193             | 0.0139             | 0.0173 | 0.00747 | 0.0284 | $2.67 \times 10^{-5}$ | 0.0652             |
|          | 8192 | 22.5 ms          | 4.09 ms   | 0.0128             | 0.00963            | 0.0107 | 0.00488 | 0.0191 | $1.92 \times 10^{-5}$ | 0.0518             |
| 0.1      | 2    | 23.2 ms          | 5.35 ms   | 972                | $2.24 \times 10^4$ | 2.19   | 0.805   | 7.31   | 0.00409               | $7 \times 10^5$    |
|          | 4    | 23.6 ms          | 5.51 ms   | 1.31               | 1.86               | 0.911  | 0.538   | 1.42   | 0.00547               | 38.2               |
|          | 8    | 23.6 ms          | 5.29 ms   | 0.613              | 0.446              | 0.513  | 0.304   | 0.816  | 0.00219               | 2.65               |
|          | 16   | 23.6 ms          | 5.48 ms   | 0.395              | 0.276              | 0.354  | 0.182   | 0.537  | 0.00131               | 1.66               |
|          | 32   | 23.5 ms          | 5.56 ms   | 0.245              | 0.176              | 0.22   | 0.1     | 0.355  | $1.34 \times 10^{-4}$ | 1.11               |
|          | 64   | 23.5 ms          | 5.43 ms   | 0.148              | 0.117              | 0.126  | 0.0533  | 0.215  | $1.59 \times 10^{-4}$ | 0.613              |
|          | 128  | 23.6 ms          | 5.64 ms   | 0.0937             | 0.0771             | 0.0733 | 0.034   | 0.134  | $8.85 \times 10^{-5}$ | 0.42               |
|          | 256  | 23.6 ms          | 5.58 ms   | 0.0658             | 0.0533             | 0.0535 | 0.0244  | 0.0937 | $1.12 \times 10^{-4}$ | 0.307              |
|          | 512  | 23.1 ms          | 5.08 ms   | 0.0478             | 0.0368             | 0.0412 | 0.0183  | 0.0689 | $4.38 \times 10^{-5}$ | 0.223              |
|          | 1024 | 23.1 ms          | 5.07 ms   | 0.0343             | 0.0261             | 0.0289 | 0.0147  | 0.0487 | $1.36 \times 10^{-4}$ | 0.154              |
|          | 2048 | 23.4 ms          | 5.44 ms   | 0.0248             | 0.0191             | 0.0209 | 0.00942 | 0.0361 | $6.14 \times 10^{-5}$ | 0.107              |
|          | 4096 | 23.6 ms          | 5.41 ms   | 0.0174             | 0.0133             | 0.0146 | 0.00705 | 0.0256 | $1.29 \times 10^{-5}$ | 0.0678             |
|          | 8192 | 23.8 ms          | 5.28 ms   | 0.0131             | 0.0095             | 0.0115 | 0.00567 | 0.0192 | $1.02 \times 10^{-5}$ | 0.0568             |
| 1        | 2    | 23 ms            | 4.99 ms   | $3.8 \times 10^5$  | $1.18 \times 10^7$ | 2.1    | 0.606   | 12.4   | 0.00213               | $3.74 \times 10^8$ |
|          | 4    | 23.2 ms          | 5.05 ms   | 2.33               | 8.2                | 0.628  | 0.264   | 1.52   | $1.76 \times 10^{-4}$ | 123                |
|          | 8    | 23.3 ms          | 5.18 ms   | 0.608              | 0.788              | 0.428  | 0.187   | 0.746  | 0.00142               | 11.3               |
|          | 16   | 23.4 ms          | 5.44 ms   | 0.379              | 0.334              | 0.295  | 0.141   | 0.527  | $2.26 \times 10^{-4}$ | 2.63               |
|          | 32   | 23.4 ms          | 5.18 ms   | 0.254              | 0.214              | 0.199  | 0.0991  | 0.359  | $5.37 \times 10^{-5}$ | 1.45               |
|          | 64   | 23.1 ms          | 5.12 ms   | 0.173              | 0.141              | 0.145  | 0.0651  | 0.244  | $6.76 \times 10^{-5}$ | 0.92               |
|          | 128  | 23 ms            | 4.84 ms   | 0.12               | 0.0929             | 0.102  | 0.0462  | 0.171  | $7.57 \times 10^{-4}$ | 0.621              |
|          | 256  | 23.3 ms          | 5.24 ms   | 0.0839             | 0.0654             | 0.0676 | 0.0314  | 0.122  | $2.63 \times 10^{-5}$ | 0.317              |
|          | 512  | 23.5 ms          | 5.4 ms    | 0.0594             | 0.0461             | 0.0497 | 0.0233  | 0.0858 | $2.13 \times 10^{-5}$ | 0.253              |
|          | 1024 | 23.5 ms          | 5.34 ms   | 0.0417             | 0.032              | 0.0355 | 0.0169  | 0.0602 | $3.46 \times 10^{-5}$ | 0.174              |
|          | 2048 | 23.5 ms          | 5.29 ms   | 0.0306             | 0.0227             | 0.0265 | 0.0123  | 0.0439 | $1.59 \times 10^{-4}$ | 0.12               |
|          | 4096 | 23.5 ms          | 5.02 ms   | 0.0208             | 0.0158             | 0.0178 | 0.00838 | 0.0296 | $3.86 \times 10^{-6}$ | 0.0956             |
|          | 8192 | 23.8 ms          | 5.24 ms   | 0.0147             | 0.011              | 0.0126 | 0.00605 | 0.0212 | $1.48 \times 10^{-5}$ | 0.0642             |
| 10       | 2    | 24 ms            | 5.55 ms   | $2.43 \times 10^5$ | $7.48 \times 10^6$ | 34.4   | 6.44    | 215    | 0.0232                | $2.37 \times 10^8$ |
|          | 4    | 24.1 ms          | 5.44 ms   | 28                 | 66.8               | 7.27   | 3.43    | 24.1   | 0.0185                | 1010               |
|          | 8    | 23.7 ms          | 5.2 ms    | 7.29               | 11.6               | 3.69   | 1.63    | 8.01   | 0.00968               | 160                |
|          | 16   | 23.7 ms          | 5.1 ms    | 3.66               | 4.3                | 2.41   | 1.11    | 4.35   | 0.0147                | 54.1               |
|          | 32   | 24 ms            | 5.49 ms   | 2.17               | 2                  | 1.61   | 0.772   | 2.98   | $3.15 \times 10^{-4}$ | 17.5               |
|          | 64   | 23.8 ms          | 5.23 ms   | 1.45               | 1.27               | 1.13   | 0.562   | 2      | 0.00408               | 9.17               |
|          | 128  | 23.7 ms          | 5.11 ms   | 0.99               | 0.789              | 0.812  | 0.38    | 1.42   | 0.00233               | 4.98               |
|          | 256  | 23.7 ms          | 5.15 ms   | 0.684              | 0.537              | 0.573  | 0.259   | 0.972  | 0.00161               | 3.79               |
|          | 512  | 23.9 ms          | 5.32 ms   | 0.485              | 0.363              | 0.413  | 0.179   | 0.688  | $3.66 \times 10^{-4}$ | 1.96               |
|          | 1024 | 23.9 ms          | 5.21 ms   | 0.333              | 0.251              | 0.283  | 0.133   | 0.479  | $3.08 \times 10^{-4}$ | 1.37               |
|          | 2048 | 23.9 ms          | 5.41 ms   | 0.233              | 0.173              | 0.196  | 0.097   | 0.332  | $1.49 \times 10^{-4}$ | 1.1                |
|          | 4096 | 24.1 ms          | 5.64 ms   | 0.164              | 0.122              | 0.14   | 0.0663  | 0.234  | $3.93 \times 10^{-5}$ | 0.703              |
|          | 8192 | 24.2 ms          | 5.3 ms    | 0.117              | 0.0879             | 0.0976 | 0.0487  | 0.171  | $2.44 \times 10^{-4}$ | 0.53               |
| 100      | 2    | 23.2 ms          | 5.21 ms   | $8.32 \times 10^4$ | $1.33 \times 10^6$ | 301    | 61.7    | 1530   | 0.0718                | $3.92 \times 10^7$ |
|          | 4    | 23.4 ms          | 5.15 ms   | 250                | 872                | 67.6   | 28      | 208    | 0.0723                | $2.04 \times 10^4$ |
|          | 8    | 23.1 ms          | 5.16 ms   | 74.1               | 111                | 38.7   | 16.2    | 88.4   | 0.0993                | 1570               |
|          | 16   | 23.5 ms          | 5.48 ms   | 38.8               | 41                 | 27     | 11.7    | 51.6   | 0.0918                | 441                |
|          | 32   | 23.4 ms          | 5.42 ms   | 24.5               | 22.3               | 19.3   | 8.96    | 31.5   | 0.0296                | 153                |
|          | 64   | 23.4 ms          | 5.45 ms   | 15.4               | 13.3               | 12.3   | 5.76    | 21.3   | 0.0242                | 101                |
|          | 128  | 23.3 ms          | 5.3 ms    | 10.4               | 8.71               | 8.25   | 3.78    | 14.6   | $3.69 \times 10^{-4}$ | 55.5               |
|          | 256  | 23.7 ms          | 5.5 ms    | 7.28               | 5.83               | 6.06   | 2.73    | 10.6   | 0.0199                | 48.8               |
|          | 512  | 23.3 ms          | 5.26 ms   | 5                  | 3.95               | 4.27   | 1.75    | 7.38   | 0.0265                | 27.8               |
|          | 1024 | 23.5 ms          | 5.3 ms    | 3.43               | 2.61               | 2.95   | 1.37    | 4.93   | $1.52 \times 10^{-4}$ | 14.6               |
|          | 2048 | 23.7 ms          | 5.68 ms   | 2.55               | 1.87               | 2.17   | 1.08    | 3.59   | 0.00236               | 10.7               |
|          | 4096 | 23.6 ms          | 5.32 ms   | 1.83               | 1.41               | 1.49   | 0.759   | 2.62   | 0.00186               | 8.56               |
|          | 8192 | 24.2 ms          | 5.69 ms   | 1.28               | 1.01               | 1.06   | 0.489   | 1.84   | 0.00423               | 5.91               |

Table 1: **Simulation study.** Results for estimator jML. Mean, standard deviation, median, [0.25, 0.75] quantile, min and max of absolute error.

| $\kappa$ | $N$  | Computation time |           | mean               | std. dev.          | median | Error   |        | min                   | max                |
|----------|------|------------------|-----------|--------------------|--------------------|--------|---------|--------|-----------------------|--------------------|
|          |      | mean             | std. dev. |                    |                    |        | 0.25    | 0.75   |                       |                    |
| 0        | 2    | 27 ms            | 6.77 ms   | 134                | 1200               | 0      | 0       | 3.51   | 0                     | $2.76 \times 10^4$ |
|          | 4    | 26.3 ms          | 6.5 ms    | 0.733              | 2.31               | 0      | 0       | 0.969  | 0                     | 53.1               |
|          | 8    | 26.1 ms          | 6.19 ms   | 0.324              | 0.505              | 0      | 0       | 0.582  | 0                     | 3.12               |
|          | 16   | 26.3 ms          | 6.16 ms   | 0.194              | 0.304              | 0      | 0       | 0.37   | 0                     | 1.47               |
|          | 32   | 26.5 ms          | 6.41 ms   | 0.125              | 0.203              | 0      | 0       | 0.236  | 0                     | 0.899              |
|          | 64   | 26.3 ms          | 6.27 ms   | 0.0933             | 0.141              | 0      | 0       | 0.189  | 0                     | 0.749              |
|          | 128  | 26.2 ms          | 6.14 ms   | 0.0653             | 0.101              | 0      | 0       | 0.133  | 0                     | 0.435              |
|          | 256  | 26.4 ms          | 6.28 ms   | 0.0442             | 0.0704             | 0      | 0       | 0.0868 | 0                     | 0.31               |
|          | 512  | 26.3 ms          | 6.1 ms    | 0.0309             | 0.0483             | 0      | 0       | 0.0649 | 0                     | 0.196              |
|          | 1024 | 26.6 ms          | 6.46 ms   | 0.0235             | 0.036              | 0      | 0       | 0.0486 | 0                     | 0.158              |
|          | 2048 | 26.5 ms          | 6.3 ms    | 0.0176             | 0.0256             | 0      | 0       | 0.0357 | 0                     | 0.111              |
|          | 4096 | 26.9 ms          | 6.54 ms   | 0.0122             | 0.018              | 0      | 0       | 0.0257 | 0                     | 0.0832             |
|          | 8192 | 26.9 ms          | 6.2 ms    | 0.00847            | 0.0125             | 0      | 0       | 0.0174 | 0                     | 0.0583             |
| 0.01     | 2    | 22.6 ms          | 5.08 ms   | 4630               | $1.31 \times 10^5$ | 0.01   | 0.01    | 3.57   | 0.01                  | $4.1 \times 10^6$  |
|          | 4    | 22.4 ms          | 4.7 ms    | 0.726              | 1.53               | 0.01   | 0.01    | 1.02   | 0.01                  | 18.2               |
|          | 8    | 22.4 ms          | 4.71 ms   | 0.337              | 0.49               | 0.01   | 0.01    | 0.662  | 0.01                  | 2.67               |
|          | 16   | 22.3 ms          | 4.62 ms   | 0.204              | 0.305              | 0.01   | 0.01    | 0.389  | 0.01                  | 1.65               |
|          | 32   | 22.6 ms          | 4.87 ms   | 0.142              | 0.203              | 0.01   | 0.01    | 0.284  | 0.01                  | 1.16               |
|          | 64   | 22.5 ms          | 4.83 ms   | 0.1                | 0.136              | 0.01   | 0.01    | 0.189  | 0.00395               | 0.583              |
|          | 128  | 22.4 ms          | 4.62 ms   | 0.078              | 0.102              | 0.01   | 0.01    | 0.141  | 0.00782               | 0.502              |
|          | 256  | 22.4 ms          | 4.83 ms   | 0.0521             | 0.0659             | 0.01   | 0.01    | 0.0936 | 0.00469               | 0.293              |
|          | 512  | 22.7 ms          | 5.2 ms    | 0.0367             | 0.0426             | 0.01   | 0.01    | 0.0598 | 0.00112               | 0.197              |
|          | 1024 | 22.2 ms          | 4.51 ms   | 0.0273             | 0.029              | 0.01   | 0.01    | 0.0413 | $6.68 \times 10^{-4}$ | 0.142              |
|          | 2048 | 22.4 ms          | 4.51 ms   | 0.0202             | 0.0183             | 0.01   | 0.01    | 0.0262 | $1.81 \times 10^{-4}$ | 0.109              |
|          | 4096 | 22.6 ms          | 4.75 ms   | 0.0155             | 0.011              | 0.01   | 0.01    | 0.018  | $3.74 \times 10^{-5}$ | 0.0617             |
|          | 8192 | 23 ms            | 4.99 ms   | 0.0123             | 0.00696            | 0.01   | 0.01    | 0.0129 | $3.82 \times 10^{-6}$ | 0.0497             |
| 0.1      | 2    | 23 ms            | 5.3 ms    | 486                | $1.12 \times 10^4$ | 0.784  | 0.1     | 3.96   | 0.1                   | $3.5 \times 10^5$  |
|          | 4    | 23.2 ms          | 5.36 ms   | 0.737              | 1.5                | 0.1    | 0.1     | 0.938  | 0.00936               | 28.7               |
|          | 8    | 23.4 ms          | 5.38 ms   | 0.358              | 0.434              | 0.1    | 0.1     | 0.513  | 0.0211                | 2.39               |
|          | 16   | 23.2 ms          | 5.14 ms   | 0.255              | 0.263              | 0.1    | 0.1     | 0.352  | 0.00427               | 1.57               |
|          | 32   | 23 ms            | 5.11 ms   | 0.181              | 0.151              | 0.1    | 0.1     | 0.24   | 0.00125               | 1.07               |
|          | 64   | 23.3 ms          | 5.15 ms   | 0.135              | 0.0889             | 0.1    | 0.1     | 0.133  | $1.3 \times 10^{-4}$  | 0.585              |
|          | 128  | 23.3 ms          | 5.22 ms   | 0.105              | 0.0563             | 0.1    | 0.1     | 0.1    | $9.78 \times 10^{-5}$ | 0.402              |
|          | 256  | 23.2 ms          | 5.42 ms   | 0.0844             | 0.0431             | 0.1    | 0.0526  | 0.1    | $4.66 \times 10^{-4}$ | 0.296              |
|          | 512  | 23.4 ms          | 5.32 ms   | 0.0604             | 0.0395             | 0.0579 | 0.0248  | 0.1    | $1.66 \times 10^{-5}$ | 0.216              |
|          | 1024 | 23.4 ms          | 5.31 ms   | 0.0409             | 0.0326             | 0.0314 | 0.0147  | 0.0594 | $7.56 \times 10^{-6}$ | 0.15               |
|          | 2048 | 23.7 ms          | 5.6 ms    | 0.0267             | 0.0218             | 0.022  | 0.00978 | 0.0377 | $1.13 \times 10^{-4}$ | 0.105              |
|          | 4096 | 23.6 ms          | 5.41 ms   | 0.0177             | 0.0136             | 0.0146 | 0.00674 | 0.0257 | $6.54 \times 10^{-5}$ | 0.0691             |
|          | 8192 | 23.8 ms          | 5.42 ms   | 0.0131             | 0.00958            | 0.0113 | 0.00571 | 0.0192 | $6.29 \times 10^{-6}$ | 0.06               |
| 1        | 2    | 23.6 ms          | 5.33 ms   | $1.9 \times 10^5$  | $5.91 \times 10^6$ | 1      | 1       | 5.98   | 0.0113                | $1.87 \times 10^8$ |
|          | 4    | 24 ms            | 5.54 ms   | 1.97               | 6.08               | 1      | 0.559   | 1.05   | 0.00152               | 91.9               |
|          | 8    | 24 ms            | 5.17 ms   | 0.649              | 0.686              | 0.499  | 0.214   | 1      | $4.43 \times 10^{-5}$ | 9.81               |
|          | 16   | 24 ms            | 5.38 ms   | 0.402              | 0.337              | 0.309  | 0.14    | 0.561  | $2.27 \times 10^{-4}$ | 2.45               |
|          | 32   | 23.7 ms          | 5.12 ms   | 0.257              | 0.212              | 0.21   | 0.0961  | 0.364  | $6.57 \times 10^{-4}$ | 1.39               |
|          | 64   | 23.6 ms          | 5.1 ms    | 0.174              | 0.139              | 0.146  | 0.0657  | 0.242  | $3.01 \times 10^{-4}$ | 0.897              |
|          | 128  | 24.1 ms          | 5.43 ms   | 0.121              | 0.0924             | 0.104  | 0.0462  | 0.175  | $3.45 \times 10^{-5}$ | 0.61               |
|          | 256  | 23.9 ms          | 5.4 ms    | 0.0839             | 0.0652             | 0.0681 | 0.0325  | 0.121  | $5.14 \times 10^{-4}$ | 0.312              |
|          | 512  | 24.1 ms          | 5.31 ms   | 0.0594             | 0.0461             | 0.0498 | 0.0235  | 0.0865 | $3.95 \times 10^{-5}$ | 0.25               |
|          | 1024 | 24.2 ms          | 5.45 ms   | 0.0417             | 0.032              | 0.0358 | 0.0171  | 0.0597 | $7.22 \times 10^{-5}$ | 0.173              |
|          | 2048 | 24.3 ms          | 5.43 ms   | 0.0306             | 0.0227             | 0.026  | 0.012   | 0.0438 | $2.45 \times 10^{-5}$ | 0.119              |
|          | 4096 | 24 ms            | 5.13 ms   | 0.0207             | 0.0158             | 0.0178 | 0.00816 | 0.0297 | $6.19 \times 10^{-5}$ | 0.0953             |
|          | 8192 | 24.1 ms          | 5.19 ms   | 0.0147             | 0.011              | 0.0125 | 0.006   | 0.0212 | $6.33 \times 10^{-6}$ | 0.064              |
| 10       | 2    | 23.7 ms          | 5.28 ms   | $1.22 \times 10^5$ | $3.74 \times 10^6$ | 12.4   | 4.84    | 103    | 0.019                 | $1.18 \times 10^8$ |
|          | 4    | 23.7 ms          | 5.37 ms   | 20.1               | 49.6               | 5.39   | 2.74    | 15.7   | 0.0316                | 752                |
|          | 8    | 23.6 ms          | 5.24 ms   | 6.13               | 9.81               | 3.35   | 1.62    | 6.15   | 0.00369               | 139                |
|          | 16   | 23.9 ms          | 5.54 ms   | 3.36               | 3.83               | 2.36   | 1.2     | 3.97   | 0.00671               | 50.1               |
|          | 32   | 23.7 ms          | 5.39 ms   | 2.07               | 1.85               | 1.6    | 0.815   | 2.8    | $2.28 \times 10^{-4}$ | 16.7               |
|          | 64   | 23.7 ms          | 5.38 ms   | 1.42               | 1.22               | 1.12   | 0.517   | 2      | 0.00247               | 8.87               |
|          | 128  | 23.8 ms          | 5.4 ms    | 0.974              | 0.772              | 0.82   | 0.362   | 1.42   | 0.00128               | 4.87               |
|          | 256  | 23.8 ms          | 5.28 ms   | 0.678              | 0.529              | 0.567  | 0.254   | 0.959  | 0.00143               | 3.73               |
|          | 512  | 23.7 ms          | 5.31 ms   | 0.483              | 0.359              | 0.42   | 0.188   | 0.688  | $4.93 \times 10^{-4}$ | 1.93               |
|          | 1024 | 23.9 ms          | 5.24 ms   | 0.332              | 0.25               | 0.282  | 0.134   | 0.477  | $1.06 \times 10^{-4}$ | 1.36               |
|          | 2048 | 23.7 ms          | 5.27 ms   | 0.233              | 0.173              | 0.196  | 0.0964  | 0.334  | $1.98 \times 10^{-4}$ | 1.09               |
|          | 4096 | 23.9 ms          | 5.22 ms   | 0.163              | 0.122              | 0.139  | 0.0679  | 0.234  | $1.15 \times 10^{-5}$ | 0.705              |
|          | 8192 | 24 ms            | 5.27 ms   | 0.117              | 0.0879             | 0.0973 | 0.049   | 0.172  | $4.64 \times 10^{-4}$ | 0.529              |
| 100      | 2    | 23.3 ms          | 5.36 ms   | $4.16 \times 10^4$ | $6.66 \times 10^5$ | 101    | 46.7    | 715    | 0.242                 | $1.96 \times 10^7$ |
|          | 4    | 23.4 ms          | 5.49 ms   | 179                | 650                | 53     | 25      | 131    | 0.103                 | $1.53 \times 10^4$ |
|          | 8    | 23.7 ms          | 5.36 ms   | 62.1               | 92.8               | 35.1   | 16.3    | 65.8   | 0.132                 | 1360               |
|          | 16   | 23.7 ms          | 5.72 ms   | 35.1               | 36.3               | 24.8   | 11.8    | 45.1   | 0.00378               | 407                |
|          | 32   | 23.4 ms          | 5.37 ms   | 23.1               | 20.8               | 18.6   | 9.07    | 29.8   | 0.0695                | 145                |
|          | 64   | 23.3 ms          | 5.4 ms    | 15.1               | 12.7               | 12.2   | 5.8     | 20.8   | 0.00212               | 97.9               |
|          | 128  | 23.3 ms          | 5.44 ms   | 10.2               | 8.49               | 8.09   | 3.69    | 14.4   | 0.00751               | 54.3               |
|          | 256  | 23.3 ms          | 5.34 ms   | 7.24               | 5.74               | 6.03   | 2.72    | 10.4   | 0.0207                | 48.2               |
|          | 512  | 23.4 ms          | 5.51 ms   | 4.98               | 3.93               | 4.32   | 1.73    | 7.35   | 0.00108               | 27.5               |
|          | 1024 | 23.5 ms          | 5.41 ms   | 3.43               | 2.6                | 2.92   | 1.39    | 4.93   | $6.36 \times 10^{-4}$ | 14.5               |
|          | 2048 | 23.7 ms          | 5.57 ms   | 2.55               | 1.87               | 2.18   | 1.08    | 3.61   | 0.00287               | 10.7               |
|          | 4096 | 23.6 ms          | 5.4 ms    | 1.83               | 1.41               | 1.48   | 0.744   | 2.62   | 0.00109               | 8.53               |
|          | 8192 | 23.6 ms          | 5.47 ms   | 1.28               | 1.01               | 1.05   | 0.491   | 1.83   | 0.0017                | 5.9                |

Table 2: **Simulation study.** Results for estimator mML. Mean, standard deviation, median, [0.25, 0.75] quantile, min and max of absolute error.

| $\kappa$ | $N$  | Computation time |           | Error              |                    |         |         |        |                       |                    |
|----------|------|------------------|-----------|--------------------|--------------------|---------|---------|--------|-----------------------|--------------------|
|          |      | mean             | std. dev. | mean               | std. dev.          | median  | 0.25    | 0.75   | min                   | max                |
| 0        | 2    | 47.6 ms          | 9.73 ms   | 27                 | 240                | 0.349   | 0       | 1.03   | 0                     | 5520               |
|          | 4    | 47.8 ms          | 8.85 ms   | 0.64               | 1.22               | 0.418   | 0       | 0.96   | 0                     | 28                 |
|          | 8    | 47.3 ms          | 8.38 ms   | 0.394              | 0.45               | 0.245   | 0       | 0.622  | 0                     | 2.28               |
|          | 16   | 47.9 ms          | 8.52 ms   | 0.231              | 0.284              | 0.122   | 0       | 0.384  | 0                     | 1.48               |
|          | 32   | 48.5 ms          | 9.16 ms   | 0.147              | 0.184              | 0.0588  | 0       | 0.247  | 0                     | 0.881              |
|          | 64   | 47.7 ms          | 8.39 ms   | 0.108              | 0.125              | 0.0604  | 0       | 0.185  | 0                     | 0.735              |
|          | 128  | 48.3 ms          | 8.75 ms   | 0.0754             | 0.089              | 0.0448  | 0       | 0.129  | 0                     | 0.42               |
|          | 256  | 47.9 ms          | 8.66 ms   | 0.05               | 0.0629             | 0.0197  | 0       | 0.0866 | 0                     | 0.299              |
|          | 512  | 47.8 ms          | 8.59 ms   | 0.0353             | 0.0428             | 0.0175  | 0       | 0.0632 | 0                     | 0.187              |
|          | 1024 | 48.5 ms          | 8.88 ms   | 0.0264             | 0.0317             | 0.0139  | 0       | 0.0464 | 0                     | 0.153              |
|          | 2048 | 48.2 ms          | 8.72 ms   | 0.0199             | 0.0224             | 0.0132  | 0       | 0.0336 | 0                     | 0.107              |
|          | 4096 | 48.6 ms          | 8.85 ms   | 0.0136             | 0.0159             | 0.0076  | 0       | 0.0241 | 0                     | 0.0805             |
|          | 8192 | 48.9 ms          | 9.25 ms   | 0.00962            | 0.011              | 0.00589 | 0       | 0.0165 | 0                     | 0.0564             |
| 0.01     | 2    | 45.6 ms          | 7.99 ms   | 927                | $2.61 \times 10^4$ | 0.351   | 0.01    | 1.08   | 0.00117               | $8.21 \times 10^5$ |
|          | 4    | 46 ms            | 8.35 ms   | 0.619              | 0.82               | 0.436   | 0.01    | 0.981  | $3.48 \times 10^{-4}$ | 9.59               |
|          | 8    | 45.7 ms          | 7.84 ms   | 0.392              | 0.452              | 0.221   | 0.01    | 0.679  | 0.00118               | 1.94               |
|          | 16   | 45.4 ms          | 8.05 ms   | 0.24               | 0.282              | 0.138   | 0.01    | 0.393  | $2.95 \times 10^{-4}$ | 1.67               |
|          | 32   | 45.6 ms          | 8.31 ms   | 0.158              | 0.183              | 0.0821  | 0.01    | 0.273  | $6.53 \times 10^{-5}$ | 1.15               |
|          | 64   | 45.9 ms          | 8.03 ms   | 0.11               | 0.122              | 0.0584  | 0.01    | 0.181  | $3.57 \times 10^{-4}$ | 0.564              |
|          | 128  | 45.9 ms          | 8.2 ms    | 0.0814             | 0.0914             | 0.0408  | 0.01    | 0.131  | $1.38 \times 10^{-4}$ | 0.489              |
|          | 256  | 45.6 ms          | 8.28 ms   | 0.0535             | 0.0593             | 0.0196  | 0.01    | 0.0873 | $1.41 \times 10^{-4}$ | 0.282              |
|          | 512  | 45.9 ms          | 8.36 ms   | 0.0365             | 0.0383             | 0.0103  | 0.01    | 0.0563 | $8.96 \times 10^{-5}$ | 0.189              |
|          | 1024 | 45.8 ms          | 8.21 ms   | 0.0261             | 0.0265             | 0.01    | 0.01    | 0.0381 | $7.53 \times 10^{-6}$ | 0.136              |
|          | 2048 | 45.4 ms          | 8.28 ms   | 0.0185             | 0.017              | 0.01    | 0.01    | 0.024  | $6.3 \times 10^{-5}$  | 0.105              |
|          | 4096 | 45.8 ms          | 7.97 ms   | 0.0134             | 0.0105             | 0.01    | 0.00814 | 0.0157 | $1.92 \times 10^{-5}$ | 0.0587             |
|          | 8192 | 46.8 ms          | 8.46 ms   | 0.0103             | 0.00705            | 0.01    | 0.00588 | 0.0106 | $2.25 \times 10^{-5}$ | 0.0478             |
| 0.1      | 2    | 46.5 ms          | 8.32 ms   | 97.2               | 2240               | 0.277   | 0.1     | 0.947  | 0.00329               | $7 \times 10^4$    |
|          | 4    | 46.6 ms          | 8.59 ms   | 0.606              | 0.787              | 0.416   | 0.1     | 0.911  | 0.0028                | 15.1               |
|          | 8    | 46.8 ms          | 8.98 ms   | 0.375              | 0.409              | 0.105   | 0.1     | 0.544  | 0.00225               | 1.77               |
|          | 16   | 46.3 ms          | 8.45 ms   | 0.251              | 0.256              | 0.1     | 0.1     | 0.341  | $3.06 \times 10^{-4}$ | 1.59               |
|          | 32   | 45.8 ms          | 8.4 ms    | 0.166              | 0.146              | 0.1     | 0.1     | 0.218  | $9.95 \times 10^{-5}$ | 1.06               |
|          | 64   | 46.3 ms          | 8.6 ms    | 0.115              | 0.0895             | 0.1     | 0.0651  | 0.116  | $1.33 \times 10^{-4}$ | 0.569              |
|          | 128  | 46.3 ms          | 8.19 ms   | 0.0862             | 0.0589             | 0.0932  | 0.0449  | 0.1    | $4.77 \times 10^{-5}$ | 0.39               |
|          | 256  | 46.3 ms          | 8.16 ms   | 0.0705             | 0.0436             | 0.0703  | 0.0346  | 0.1    | $3.81 \times 10^{-5}$ | 0.288              |
|          | 512  | 46.8 ms          | 8.43 ms   | 0.0536             | 0.0366             | 0.0481  | 0.0218  | 0.0863 | $2.56 \times 10^{-4}$ | 0.21               |
|          | 1024 | 46.7 ms          | 8.64 ms   | 0.0385             | 0.0298             | 0.0313  | 0.0148  | 0.0563 | $1.82 \times 10^{-5}$ | 0.147              |
|          | 2048 | 46.9 ms          | 8.58 ms   | 0.027              | 0.0211             | 0.0223  | 0.0102  | 0.039  | $2.66 \times 10^{-5}$ | 0.102              |
|          | 4096 | 46.7 ms          | 8.44 ms   | 0.0181             | 0.0139             | 0.0146  | 0.00714 | 0.0264 | $4.79 \times 10^{-6}$ | 0.072              |
|          | 8192 | 47 ms            | 8.45 ms   | 0.0132             | 0.00967            | 0.0112  | 0.00528 | 0.0193 | $6.52 \times 10^{-5}$ | 0.0624             |
| 1        | 2    | 47.5 ms          | 8.89 ms   | $3.8 \times 10^4$  | $1.18 \times 10^6$ | 0.771   | 0.453   | 1      | 0.00269               | $3.74 \times 10^7$ |
|          | 4    | 47.1 ms          | 8.29 ms   | 0.998              | 3.14               | 0.506   | 0.182   | 0.979  | $6.24 \times 10^{-4}$ | 48.1               |
|          | 8    | 47.8 ms          | 8.79 ms   | 0.518              | 0.475              | 0.439   | 0.219   | 0.73   | 0.00161               | 7.1                |
|          | 16   | 47.9 ms          | 9.02 ms   | 0.389              | 0.288              | 0.327   | 0.153   | 0.57   | $8.39 \times 10^{-4}$ | 1.98               |
|          | 32   | 47.6 ms          | 8.64 ms   | 0.265              | 0.21               | 0.219   | 0.101   | 0.373  | $9.97 \times 10^{-4}$ | 1.22               |
|          | 64   | 48 ms            | 8.95 ms   | 0.178              | 0.141              | 0.15    | 0.0663  | 0.25   | $9.96 \times 10^{-5}$ | 0.904              |
|          | 128  | 47.5 ms          | 8.41 ms   | 0.122              | 0.0932             | 0.105   | 0.0468  | 0.178  | $1.47 \times 10^{-4}$ | 0.611              |
|          | 256  | 47.7 ms          | 8.71 ms   | 0.0844             | 0.0654             | 0.0677  | 0.0321  | 0.123  | $1.41 \times 10^{-4}$ | 0.311              |
|          | 512  | 47.7 ms          | 8.41 ms   | 0.0596             | 0.0461             | 0.0495  | 0.0238  | 0.087  | $2.91 \times 10^{-5}$ | 0.25               |
|          | 1024 | 47.7 ms          | 8.6 ms    | 0.0417             | 0.032              | 0.0359  | 0.0166  | 0.0599 | $7.25 \times 10^{-6}$ | 0.173              |
|          | 2048 | 48.1 ms          | 9.02 ms   | 0.0306             | 0.0227             | 0.0262  | 0.0121  | 0.0438 | $1.49 \times 10^{-4}$ | 0.119              |
|          | 4096 | 48.3 ms          | 8.72 ms   | 0.0207             | 0.0158             | 0.0177  | 0.00811 | 0.0297 | $7.63 \times 10^{-6}$ | 0.0951             |
|          | 8192 | 48.9 ms          | 9.03 ms   | 0.0147             | 0.011              | 0.0125  | 0.00599 | 0.0212 | $5.25 \times 10^{-6}$ | 0.0639             |
| 10       | 2    | 46.5 ms          | 8.5 ms    | $2.43 \times 10^4$ | $7.48 \times 10^5$ | 8.6     | 6.2     | 12.5   | 0.0121                | $2.37 \times 10^7$ |
|          | 4    | 46 ms            | 8.11 ms   | 11                 | 24.8               | 5.7     | 3.25    | 7.79   | 0.0282                | 393                |
|          | 8    | 46.9 ms          | 8.42 ms   | 4.94               | 6.63               | 3.65    | 1.98    | 5.45   | 0.0065                | 102                |
|          | 16   | 46.8 ms          | 8.65 ms   | 3.07               | 3.01               | 2.52    | 1.29    | 3.9    | $1.87 \times 10^{-4}$ | 42.6               |
|          | 32   | 46.4 ms          | 8.4 ms    | 1.99               | 1.6                | 1.68    | 0.815   | 2.77   | 0.00126               | 15                 |
|          | 64   | 46.6 ms          | 8.55 ms   | 1.39               | 1.13               | 1.15    | 0.526   | 2      | $4.68 \times 10^{-4}$ | 8.28               |
|          | 128  | 46.1 ms          | 8.16 ms   | 0.954              | 0.744              | 0.788   | 0.373   | 1.38   | $2.59 \times 10^{-4}$ | 4.63               |
|          | 256  | 46.7 ms          | 8.52 ms   | 0.668              | 0.518              | 0.573   | 0.267   | 0.957  | $9.99 \times 10^{-5}$ | 3.62               |
|          | 512  | 46.5 ms          | 8.01 ms   | 0.481              | 0.353              | 0.429   | 0.196   | 0.691  | $3.42 \times 10^{-5}$ | 1.89               |
|          | 1024 | 46.4 ms          | 8.39 ms   | 0.331              | 0.249              | 0.281   | 0.134   | 0.474  | $5.73 \times 10^{-5}$ | 1.34               |
|          | 2048 | 46.6 ms          | 8.61 ms   | 0.233              | 0.173              | 0.197   | 0.0976  | 0.334  | 0.00198               | 1.08               |
|          | 4096 | 46.8 ms          | 8.77 ms   | 0.163              | 0.122              | 0.138   | 0.0688  | 0.233  | $2.06 \times 10^{-5}$ | 0.71               |
|          | 8192 | 46.9 ms          | 8.65 ms   | 0.117              | 0.0878             | 0.0971  | 0.0489  | 0.172  | $4.59 \times 10^{-6}$ | 0.527              |
| 100      | 2    | 46.1 ms          | 8.28 ms   | 8320               | $1.33 \times 10^5$ | 83.9    | 60.1    | 96.1   | 0.0532                | $3.92 \times 10^6$ |
|          | 4    | 46.5 ms          | 8.14 ms   | 101                | 335                | 54.7    | 31.5    | 75.6   | 0.0137                | 8050               |
|          | 8    | 46.6 ms          | 8.52 ms   | 48.9               | 62.2               | 37.1    | 20      | 56.1   | 0.0231                | 1000               |
|          | 16   | 47.2 ms          | 8.87 ms   | 30.8               | 28                 | 25.2    | 12.8    | 41     | 0.0423                | 344                |
|          | 32   | 46.6 ms          | 8.2 ms    | 21.4               | 18                 | 17.5    | 8.54    | 28.5   | 0.0306                | 130                |
|          | 64   | 46.6 ms          | 8.35 ms   | 14.7               | 11.7               | 12.5    | 5.91    | 20.9   | 0.016                 | 91.8               |
|          | 128  | 46.6 ms          | 8.36 ms   | 10.1               | 8.11               | 8.26    | 3.86    | 14.3   | 0.012                 | 51.9               |
|          | 256  | 46.8 ms          | 8.48 ms   | 7.2                | 5.61               | 6.14    | 2.85    | 10.3   | $3.33 \times 10^{-4}$ | 47                 |
|          | 512  | 46 ms            | 8.04 ms   | 4.96               | 3.88               | 4.31    | 1.77    | 7.3    | 0.0104                | 27                 |
|          | 1024 | 46.1 ms          | 8.14 ms   | 3.43               | 2.59               | 2.91    | 1.37    | 4.83   | 0.0211                | 14.2               |
|          | 2048 | 46.8 ms          | 8.36 ms   | 2.55               | 1.86               | 2.17    | 1.07    | 3.66   | $2.48 \times 10^{-5}$ | 10.6               |
|          | 4096 | 46.7 ms          | 8.46 ms   | 1.83               | 1.41               | 1.47    | 0.742   | 2.65   | $7.36 \times 10^{-4}$ | 8.48               |
|          | 8192 | 47.2 ms          | 8.52 ms   | 1.28               | 1.01               | 1.05    | 0.493   | 1.82   | 0.00336               | 5.87               |

Table 3: **Simulation study.** Results for estimator BF1. Mean, standard deviation, median, [0.25, 0.75] quantile, min and max of absolute error.

| $\kappa$ | $N$  | Computation time |           | Error  |                        |        | 0.25                  | 0.75   | min                   | max    |
|----------|------|------------------|-----------|--------|------------------------|--------|-----------------------|--------|-----------------------|--------|
|          |      | mean             | std. dev. | mean   | std. dev.              | median |                       |        |                       |        |
| 0        | 2    | 93.4 ms          | 15.4 ms   | 0      | 0                      | 0      | 0                     | 0      | 0                     | 0      |
|          | 4    | 141 ms           | 17.2 ms   | 0.0924 | 0.473                  | 0      | 0                     | 0      | 0                     | 12.6   |
|          | 8    | 233 ms           | 23.4 ms   | 0.351  | 0.34                   | 0.31   | 0                     | 0.547  | 0                     | 1.84   |
|          | 16   | 423 ms           | 30.6 ms   | 0.277  | 0.266                  | 0.223  | $1.55 \times 10^{-4}$ |        | 0.438                 | 1.36   |
|          | 32   | 796 ms           | 43 ms     | 0.194  | 0.186                  | 0.16   | 0                     | 0.311  | 0                     | 0.871  |
|          | 64   | 1.55 s           | 61.3 ms   | 0.149  | 0.128                  | 0.131  | 0.0304                | 0.232  | 0                     | 0.738  |
|          | 128  | 3.05 s           | 89.8 ms   | 0.105  | 0.0925                 | 0.096  | 0.0166                | 0.165  | 0                     | 0.433  |
|          | 256  | 6.06 s           | 137 ms    | 0.0709 | 0.0662                 | 0.0601 | 0.00402               | 0.114  | 0                     | 0.31   |
|          | 512  | 12.1 s           | 216 ms    | 0.0502 | 0.0455                 | 0.0445 | 0.00292               | 0.082  | 0                     | 0.197  |
|          | 1024 | 24.2 s           | 347 ms    | 0.0374 | 0.0332                 | 0.0326 | 0.00523               | 0.0598 | 0                     | 0.158  |
|          | 2048 | 48.4 s           | 524 ms    | 0.0276 | 0.0236                 | 0.0261 | 0.00437               | 0.043  | 0                     | 0.111  |
|          | 4096 | 97.1 s           | 879 ms    | 0.0192 | 0.0166                 | 0.0169 | 0.00282               | 0.0306 | 0                     | 0.0833 |
|          | 8192 | 196 s            | 1.6 s     | 0.0136 | 0.0115                 | 0.0123 | 0.00205               | 0.0212 | 0                     | 0.0584 |
| 0.01     | 2    | 93.3 ms          | 13.1 ms   | 0.01   | $1.68 \times 10^{-16}$ | 0.01   | 0.01                  | 0.01   | 0.01                  | 0.01   |
|          | 4    | 141 ms           | 17.8 ms   | 0.107  | 0.39                   | 0.01   | 0.01                  | 0.01   | 0.00141               | 6.47   |
|          | 8    | 235 ms           | 22.6 ms   | 0.345  | 0.336                  | 0.285  | 0.01                  | 0.579  | $1.26 \times 10^{-5}$ | 2.19   |
|          | 16   | 424 ms           | 30.7 ms   | 0.284  | 0.264                  | 0.246  | 0.01                  | 0.442  | 0.00153               | 1.51   |
|          | 32   | 800 ms           | 44.7 ms   | 0.203  | 0.185                  | 0.173  | 0.01                  | 0.328  | $2.35 \times 10^{-4}$ | 1.12   |
|          | 64   | 1.55 s           | 60.5 ms   | 0.146  | 0.127                  | 0.127  | 0.0156                | 0.228  | $4.55 \times 10^{-4}$ | 0.579  |
|          | 128  | 3.06 s           | 95.5 ms   | 0.107  | 0.0961                 | 0.0902 | 0.01                  | 0.166  | $4.51 \times 10^{-5}$ | 0.5    |
|          | 256  | 6.06 s           | 134 ms    | 0.0717 | 0.0631                 | 0.0573 | 0.01                  | 0.113  | $2.65 \times 10^{-5}$ | 0.293  |
|          | 512  | 12.1 s           | 204 ms    | 0.048  | 0.0422                 | 0.0366 | 0.01                  | 0.0746 | $1.41 \times 10^{-4}$ | 0.197  |
|          | 1024 | 24.2 s           | 302 ms    | 0.0337 | 0.0291                 | 0.0249 | 0.01                  | 0.0512 | $3.47 \times 10^{-6}$ | 0.142  |
|          | 2048 | 48.4 s           | 451 ms    | 0.0228 | 0.0193                 | 0.0145 | 0.01                  | 0.0332 | $2.23 \times 10^{-5}$ | 0.109  |
|          | 4096 | 97.2 s           | 703 ms    | 0.0156 | 0.0123                 | 0.01   | 0.00774               | 0.0221 | $7.02 \times 10^{-5}$ | 0.0619 |
|          | 8192 | 196 s            | 1.23 s    | 0.0111 | 0.00831                | 0.01   | 0.00499               | 0.0148 | $6.93 \times 10^{-6}$ | 0.0498 |
| 0.1      | 2    | 93.6 ms          | 13.1 ms   | 0.1    | $1.42 \times 10^{-15}$ | 0.1    | 0.1                   | 0.1    | 0.1                   | 0.1    |
|          | 4    | 141 ms           | 16.8 ms   | 0.189  | 0.632                  | 0.1    | 0.1                   | 0.1    | $6.65 \times 10^{-4}$ | 16.1   |
|          | 8    | 233 ms           | 22 ms     | 0.306  | 0.302                  | 0.159  | 0.1                   | 0.456  | 0.00104               | 2.14   |
|          | 16   | 423 ms           | 30.3 ms   | 0.267  | 0.241                  | 0.169  | 0.1                   | 0.379  | $4.33 \times 10^{-4}$ | 1.41   |
|          | 32   | 799 ms           | 43.3 ms   | 0.185  | 0.154                  | 0.111  | 0.0912                | 0.266  | $9.69 \times 10^{-5}$ | 1.03   |
|          | 64   | 1.55 s           | 60 ms     | 0.124  | 0.0997                 | 0.1    | 0.0568                | 0.159  | $2.38 \times 10^{-4}$ | 0.576  |
|          | 128  | 3.06 s           | 87.9 ms   | 0.0867 | 0.0665                 | 0.0816 | 0.0363                | 0.1    | $1.92 \times 10^{-5}$ | 0.4    |
|          | 256  | 6.05 s           | 139 ms    | 0.0676 | 0.0472                 | 0.0613 | 0.0304                | 0.1    | $6.7 \times 10^{-5}$  | 0.296  |
|          | 512  | 12.1 s           | 209 ms    | 0.0504 | 0.0372                 | 0.0433 | 0.0193                | 0.0776 | $4.69 \times 10^{-6}$ | 0.216  |
|          | 1024 | 24.1 s           | 312 ms    | 0.0362 | 0.0279                 | 0.0294 | 0.0142                | 0.0517 | $9.76 \times 10^{-6}$ | 0.15   |
|          | 2048 | 48.3 s           | 456 ms    | 0.0256 | 0.0199                 | 0.0217 | 0.00958               | 0.0371 | $9.67 \times 10^{-6}$ | 0.105  |
|          | 4096 | 97.1 s           | 650 ms    | 0.0177 | 0.0135                 | 0.0146 | 0.00672               | 0.0257 | $5.38 \times 10^{-5}$ | 0.0663 |
|          | 8192 | 196 s            | 1.11 s    | 0.0131 | 0.00957                | 0.0113 | 0.00572               | 0.0192 | $6.88 \times 10^{-6}$ | 0.0596 |
| 1        | 2    | 93.9 ms          | 13.5 ms   | 1      | 0                      | 1      | 1                     | 1      | 1                     | 1      |
|          | 4    | 141 ms           | 17.6 ms   | 0.943  | 0.605                  | 1      | 1                     | 1      | 0.00276               | 16.4   |
|          | 8    | 237 ms           | 24.6 ms   | 0.463  | 0.385                  | 0.375  | 0.207                 | 0.66   | $1.71 \times 10^{-4}$ | 4.81   |
|          | 16   | 424 ms           | 32.5 ms   | 0.335  | 0.261                  | 0.288  | 0.129                 | 0.474  | 0.00115               | 1.95   |
|          | 32   | 804 ms           | 44.8 ms   | 0.244  | 0.193                  | 0.204  | 0.0915                | 0.343  | $2.68 \times 10^{-4}$ | 1.29   |
|          | 64   | 1.56 s           | 63.6 ms   | 0.17   | 0.134                  | 0.145  | 0.0638                | 0.24   | $3.67 \times 10^{-5}$ | 0.853  |
|          | 128  | 3.08 s           | 96.2 ms   | 0.119  | 0.0911                 | 0.102  | 0.046                 | 0.175  | $3.19 \times 10^{-4}$ | 0.595  |
|          | 256  | 6.12 s           | 158 ms    | 0.0835 | 0.0647                 | 0.0664 | 0.0317                | 0.122  | $1.66 \times 10^{-5}$ | 0.307  |
|          | 512  | 12.2 s           | 255 ms    | 0.0593 | 0.0459                 | 0.049  | 0.0236                | 0.0861 | $1.98 \times 10^{-4}$ | 0.248  |
|          | 1024 | 24.4 s           | 412 ms    | 0.0416 | 0.032                  | 0.036  | 0.0164                | 0.0599 | $1.99 \times 10^{-5}$ | 0.172  |
|          | 2048 | 48.8 s           | 711 ms    | 0.0305 | 0.0227                 | 0.0262 | 0.0121                | 0.0437 | $1.86 \times 10^{-4}$ | 0.119  |
|          | 4096 | 98 s             | 1.26 s    | 0.0207 | 0.0158                 | 0.0177 | 0.00807               | 0.0297 | $4.97 \times 10^{-5}$ | 0.095  |
|          | 8192 | 198 s            | 2.32 s    | 0.0147 | 0.011                  | 0.0125 | 0.00597               | 0.0212 | $3.22 \times 10^{-5}$ | 0.0639 |
| 10       | 2    | 93.2 ms          | 13 ms     | 10     | 0                      | 10     | 10                    | 10     | 10                    | 10     |
|          | 4    | 142 ms           | 17.1 ms   | 9.9    | 9.05                   | 10     | 10                    | 10     | 0.0612                | 151    |
|          | 8    | 234 ms           | 22.1 ms   | 5.84   | 5.52                   | 4.95   | 2.8                   | 7.79   | 0.00658               | 74.8   |
|          | 16   | 425 ms           | 31.4 ms   | 3.23   | 2.87                   | 2.72   | 1.46                  | 4.33   | $3.39 \times 10^{-4}$ | 41.5   |
|          | 32   | 802 ms           | 42.4 ms   | 1.99   | 1.56                   | 1.72   | 0.823                 | 2.77   | 0.00746               | 13.2   |
|          | 64   | 1.56 s           | 63.4 ms   | 1.39   | 1.12                   | 1.15   | 0.529                 | 1.98   | 0.00267               | 8.41   |
|          | 128  | 3.08 s           | 91.3 ms   | 0.953  | 0.743                  | 0.794  | 0.368                 | 1.38   | $5.09 \times 10^{-4}$ | 4.69   |
|          | 256  | 6.12 s           | 142 ms    | 0.668  | 0.518                  | 0.573  | 0.271                 | 0.964  | 0.00144               | 3.64   |
|          | 512  | 12.2 s           | 230 ms    | 0.481  | 0.353                  | 0.429  | 0.195                 | 0.693  | $2.91 \times 10^{-4}$ | 1.9    |
|          | 1024 | 24.3 s           | 388 ms    | 0.331  | 0.249                  | 0.282  | 0.133                 | 0.473  | $1.64 \times 10^{-4}$ | 1.33   |
|          | 2048 | 48.7 s           | 682 ms    | 0.233  | 0.173                  | 0.196  | 0.0975                | 0.334  | 0.00203               | 1.08   |
|          | 4096 | 97.6 s           | 1.23 s    | 0.163  | 0.122                  | 0.138  | 0.0686                | 0.233  | $1.62 \times 10^{-4}$ | 0.709  |
|          | 8192 | 197 s            | 2.26 s    | 0.117  | 0.0878                 | 0.0971 | 0.0491                | 0.172  | $7.96 \times 10^{-5}$ | 0.527  |
| 100      | 2    | 94.6 ms          | 13.1 ms   | 100    | 0                      | 100    | 100                   | 100    | 100                   | 100    |
|          | 4    | 142 ms           | 17 ms     | 96.6   | 67.8                   | 100    | 100                   | 100    | 0.101                 | 1680   |
|          | 8    | 237 ms           | 24.5 ms   | 60.4   | 51                     | 53.6   | 27.8                  | 83.2   | 0.0578                | 513    |
|          | 16   | 428 ms           | 36.1 ms   | 33     | 28.6                   | 27.5   | 13.5                  | 44     | 0.0727                | 374    |
|          | 32   | 808 ms           | 52.1 ms   | 21.5   | 17.9                   | 17.7   | 8.57                  | 29.5   | 0.0232                | 128    |
|          | 64   | 1.57 s           | 83.7 ms   | 14.6   | 11.6                   | 12.3   | 5.93                  | 20.9   | 0.0493                | 94.1   |
|          | 128  | 3.1 s            | 144 ms    | 10     | 8.11                   | 8.34   | 3.84                  | 14.3   | $6.33 \times 10^{-4}$ | 52.7   |
|          | 256  | 6.15 s           | 249 ms    | 7.2    | 5.61                   | 6.15   | 2.82                  | 10.2   | 0.00712               | 47     |
|          | 512  | 12.2 s           | 451 ms    | 4.96   | 3.88                   | 4.3    | 1.76                  | 7.28   | 0.0156                | 27.1   |
|          | 1024 | 24.4 s           | 909 ms    | 3.43   | 2.58                   | 2.91   | 1.37                  | 4.83   | 0.0114                | 14.2   |
|          | 2048 | 49.2 s           | 1.85 s    | 2.55   | 1.86                   | 2.17   | 1.08                  | 3.66   | $4.43 \times 10^{-4}$ | 10.6   |
|          | 4096 | 98.1 s           | 3.37 s    | 1.83   | 1.41                   | 1.48   | 0.742                 | 2.65   | $6.61 \times 10^{-4}$ | 8.48   |
|          | 8192 | 198 s            | 6.71 s    | 1.28   | 1.01                   | 1.05   | 0.493                 | 1.82   | 0.00379               | 5.87   |

Table 4: **Simulation study.** Results for estimator BF2. Mean, standard deviation, median, [0.25, 0.75] quantile, min and max of absolute error.

| $\kappa$ | $N$  | Computation time |           | mean               | std. dev.          | median | Error |       | min                   | max                |
|----------|------|------------------|-----------|--------------------|--------------------|--------|-------|-------|-----------------------|--------------------|
|          |      | mean             | std. dev. |                    |                    |        | 0.25  | 0.75  |                       |                    |
| 0        | 2    | 23.9 ms          | 8.22 ms   | 116                | 1050               | 0.677  | 0.335 | 2.56  | 0.227                 | $2.51 \times 10^4$ |
|          | 4    | 22.1 ms          | 4.37 ms   | 3.09               | 23                 | 0.531  | 0.302 | 1.17  | 0.175                 | 503                |
|          | 8    | 22.5 ms          | 4.19 ms   | 0.623              | 0.788              | 0.379  | 0.265 | 0.654 | 0.167                 | 11.4               |
|          | 16   | 22.3 ms          | 3.79 ms   | 0.378              | 0.222              | 0.306  | 0.243 | 0.43  | 0.167                 | 1.94               |
|          | 32   | 22.4 ms          | 3.93 ms   | 0.299              | 0.0928             | 0.269  | 0.235 | 0.338 | 0.181                 | 1.24               |
|          | 64   | 22.8 ms          | 4.25 ms   | 0.27               | 0.0515             | 0.258  | 0.232 | 0.296 | 0.19                  | 0.534              |
|          | 128  | 23.9 ms          | 3.96 ms   | 0.255              | 0.032              | 0.247  | 0.23  | 0.271 | 0.2                   | 0.476              |
|          | 256  | 28.9 ms          | 5.04 ms   | 0.244              | 0.0203             | 0.241  | 0.229 | 0.255 | 0.204                 | 0.355              |
|          | 512  | 47.5 ms          | 5.19 ms   | 0.239              | 0.0134             | 0.236  | 0.228 | 0.247 | 0.215                 | 0.29               |
|          | 1024 | 125 ms           | 6.62 ms   | 0.235              | 0.00926            | 0.233  | 0.228 | 0.241 | 0.218                 | 0.272              |
|          | 2048 | 493 ms           | 28.5 ms   | 0.233              | 0.00645            | 0.232  | 0.228 | 0.237 | 0.217                 | 0.26               |
|          | 4096 | 2.34 s           | 69.4 ms   | 0.231              | 0.00425            | 0.23   | 0.227 | 0.234 | 0.221                 | 0.245              |
|          | 8192 | 9.96 s           | 160 ms    | 0.23               | 0.00313            | 0.229  | 0.227 | 0.232 | 0.221                 | 0.242              |
| 0.01     | 2    | 29.7 ms          | 7.67 ms   | 4000               | $1.18 \times 10^5$ | 0.738  | 0.339 | 2.65  | 0.218                 | $3.73 \times 10^6$ |
|          | 4    | 23.7 ms          | 5.18 ms   | 6.5                | 119                | 0.529  | 0.294 | 1.27  | 0.17                  | 3720               |
|          | 8    | 23.8 ms          | 4.94 ms   | 0.651              | 1.12               | 0.38   | 0.255 | 0.645 | 0.153                 | 23.3               |
|          | 16   | 23.5 ms          | 4.86 ms   | 0.376              | 0.231              | 0.303  | 0.237 | 0.432 | 0.161                 | 2.85               |
|          | 32   | 23.4 ms          | 4.8 ms    | 0.299              | 0.107              | 0.269  | 0.228 | 0.331 | 0.169                 | 1.06               |
|          | 64   | 23.9 ms          | 5.22 ms   | 0.262              | 0.0533             | 0.248  | 0.222 | 0.289 | 0.182                 | 0.586              |
|          | 128  | 25.2 ms          | 5.55 ms   | 0.246              | 0.0346             | 0.235  | 0.22  | 0.261 | 0.189                 | 0.42               |
|          | 256  | 29.6 ms          | 5.66 ms   | 0.235              | 0.0203             | 0.23   | 0.219 | 0.246 | 0.196                 | 0.355              |
|          | 512  | 48.8 ms          | 6.29 ms   | 0.23               | 0.0137             | 0.227  | 0.218 | 0.238 | 0.202                 | 0.28               |
|          | 1024 | 129 ms           | 7.49 ms   | 0.225              | 0.00969            | 0.223  | 0.218 | 0.231 | 0.205                 | 0.267              |
|          | 2048 | 486 ms           | 21.7 ms   | 0.223              | 0.00642            | 0.221  | 0.218 | 0.227 | 0.209                 | 0.246              |
|          | 4096 | 2.33 s           | 89.8 ms   | 0.221              | 0.00452            | 0.22   | 0.217 | 0.224 | 0.212                 | 0.236              |
|          | 8192 | 10 s             | 336 ms    | 0.22               | 0.00333            | 0.219  | 0.217 | 0.222 | 0.212                 | 0.232              |
| 0.1      | 2    | 31.3 ms          | 7.71 ms   | 441                | $1.02 \times 10^4$ | 0.753  | 0.278 | 3.08  | 0.128                 | $3.19 \times 10^5$ |
|          | 4    | 24.3 ms          | 4.94 ms   | 3.78               | 50.2               | 0.495  | 0.217 | 1.16  | 0.0786                | 1550               |
|          | 8    | 24.5 ms          | 4.8 ms    | 0.537              | 0.834              | 0.287  | 0.17  | 0.556 | 0.061                 | 10.2               |
|          | 16   | 24.5 ms          | 4.93 ms   | 0.3                | 0.279              | 0.214  | 0.148 | 0.347 | 0.0641                | 3.69               |
|          | 32   | 24.5 ms          | 5.08 ms   | 0.218              | 0.116              | 0.182  | 0.139 | 0.258 | 0.0784                | 1.04               |
|          | 64   | 24.6 ms          | 4.91 ms   | 0.176              | 0.0591             | 0.158  | 0.131 | 0.204 | 0.0858                | 0.522              |
|          | 128  | 26.1 ms          | 5.5 ms    | 0.16               | 0.0377             | 0.151  | 0.13  | 0.179 | 0.103                 | 0.37               |
|          | 256  | 31 ms            | 5.99 ms   | 0.151              | 0.0271             | 0.144  | 0.129 | 0.167 | 0.112                 | 0.274              |
|          | 512  | 49.8 ms          | 6.25 ms   | 0.148              | 0.0212             | 0.144  | 0.128 | 0.162 | 0.113                 | 0.216              |
|          | 1024 | 129 ms           | 7.01 ms   | 0.144              | 0.0172             | 0.14   | 0.128 | 0.157 | 0.121                 | 0.21               |
|          | 2048 | 552 ms           | 58.1 ms   | 0.142              | 0.0151             | 0.14   | 0.128 | 0.155 | 0.122                 | 0.19               |
|          | 4096 | 2.39 s           | 252 ms    | 0.142              | 0.014              | 0.145  | 0.128 | 0.154 | 0.125                 | 0.173              |
|          | 8192 | 10.1 s           | 373 ms    | 0.141              | 0.0134             | 0.146  | 0.127 | 0.154 | 0.126                 | 0.169              |
| 1        | 2    | 30.6 ms          | 7.87 ms   | $1.73 \times 10^5$ | $5.37 \times 10^6$ | 0.73   | 0.486 | 4.72  | 0.00144               | $1.7 \times 10^8$  |
|          | 4    | 23.8 ms          | 5.4 ms    | 7                  | 45.2               | 0.678  | 0.355 | 2.01  | 0.00408               | 1190               |
|          | 8    | 24 ms            | 4.95 ms   | 1.11               | 3.25               | 0.555  | 0.287 | 0.798 | $2.79 \times 10^{-4}$ | 64.7               |
|          | 16   | 24 ms            | 5.11 ms   | 0.567              | 0.608              | 0.459  | 0.235 | 0.717 | 0.00197               | 5.93               |
|          | 32   | 24.3 ms          | 5.23 ms   | 0.383              | 0.274              | 0.341  | 0.177 | 0.522 | 0.0025                | 2.64               |
|          | 64   | 24.4 ms          | 5.47 ms   | 0.328              | 0.218              | 0.297  | 0.161 | 0.442 | $7.36 \times 10^{-4}$ | 1.41               |
|          | 128  | 25.4 ms          | 5.2 ms    | 0.31               | 0.208              | 0.28   | 0.165 | 0.389 | 0.00133               | 0.782              |
|          | 256  | 30.4 ms          | 6.24 ms   | 0.317              | 0.198              | 0.275  | 0.192 | 0.365 | 0.00123               | 0.782              |
|          | 512  | 48.9 ms          | 6.65 ms   | 0.313              | 0.174              | 0.273  | 0.22  | 0.335 | 0.00126               | 0.775              |
|          | 1024 | 133 ms           | 8.92 ms   | 0.323              | 0.171              | 0.275  | 0.233 | 0.321 | 0.0949                | 0.774              |
|          | 2048 | 629 ms           | 20.5 ms   | 0.329              | 0.177              | 0.27   | 0.241 | 0.303 | 0.127                 | 0.773              |
|          | 4096 | 2.6 s            | 96.6 ms   | 0.317              | 0.157              | 0.269  | 0.25  | 0.29  | 0.148                 | 0.773              |
|          | 8192 | 10.8 s           | 678 ms    | 0.322              | 0.159              | 0.27   | 0.256 | 0.285 | 0.174                 | 0.773              |
| 10       | 2    | 29.5 ms          | 7.17 ms   | $1.11 \times 10^5$ | $3.4 \times 10^6$  | 9.59   | 5.19  | 84.9  | 0.0375                | $1.08 \times 10^8$ |
|          | 4    | 23.6 ms          | 5.32 ms   | 190                | 2940               | 8.33   | 3.71  | 39    | 0.00434               | $9.18 \times 10^4$ |
|          | 8    | 23.8 ms          | 4.97 ms   | 16.1               | 38                 | 5.3    | 2.56  | 14.3  | 0.00253               | 575                |
|          | 16   | 23.5 ms          | 4.76 ms   | 7.6                | 12.6               | 3.84   | 1.87  | 7.26  | 0.00728               | 196                |
|          | 32   | 23.5 ms          | 4.83 ms   | 4                  | 4.45               | 2.8    | 1.37  | 4.7   | 0.0147                | 37.4               |
|          | 64   | 23.6 ms          | 4.82 ms   | 2.55               | 2.27               | 2.11   | 1.03  | 3.3   | 0.00117               | 20.8               |
|          | 128  | 24.7 ms          | 5.04 ms   | 1.67               | 1.41               | 1.35   | 0.641 | 2.3   | 0.00196               | 10.3               |
|          | 256  | 29.3 ms          | 5.77 ms   | 1.14               | 0.931              | 0.955  | 0.418 | 1.61  | 0.00396               | 6.81               |
|          | 512  | 45.9 ms          | 6.58 ms   | 0.79               | 0.589              | 0.647  | 0.347 | 1.15  | $1.15 \times 10^{-4}$ | 3.37               |
|          | 1024 | 122 ms           | 7.53 ms   | 0.573              | 0.427              | 0.487  | 0.236 | 0.817 | 0.00334               | 2.57               |
|          | 2048 | 460 ms           | 60.8 ms   | 0.45               | 0.328              | 0.383  | 0.186 | 0.656 | $4.83 \times 10^{-4}$ | 1.76               |
|          | 4096 | 1.8 s            | 153 ms    | 0.363              | 0.252              | 0.325  | 0.162 | 0.516 | $4.01 \times 10^{-4}$ | 1.56               |
|          | 8192 | 8.83 s           | 458 ms    | 0.288              | 0.198              | 0.258  | 0.127 | 0.409 | $2.3 \times 10^{-5}$  | 0.967              |
| 100      | 2    | 30.4 ms          | 8.28 ms   | $3.7 \times 10^4$  | $6.06 \times 10^5$ | 84.7   | 47.2  | 605   | 0.359                 | $1.79 \times 10^7$ |
|          | 4    | 29 ms            | 6.57 ms   | 4970               | $1.11 \times 10^5$ | 75.6   | 35.9  | 327   | 0.672                 | $3.32 \times 10^6$ |
|          | 8    | 28.9 ms          | 5.95 ms   | 150                | 374                | 52.6   | 26.1  | 134   | 0.0257                | 5310               |
|          | 16   | 28.9 ms          | 5.98 ms   | 68.4               | 98.1               | 38.3   | 18.4  | 72.4  | 0.00758               | 996                |
|          | 32   | 29.3 ms          | 5.91 ms   | 41.5               | 45.6               | 27.7   | 13.2  | 51.1  | 0.0369                | 478                |
|          | 64   | 29.2 ms          | 5.95 ms   | 25.9               | 25.1               | 19.7   | 9.05  | 34    | 0.0493                | 268                |
|          | 128  | 29.9 ms          | 6.04 ms   | 17.4               | 14.8               | 13.8   | 7.02  | 23.6  | 0.0147                | 115                |
|          | 256  | 33.7 ms          | 6.56 ms   | 11.8               | 10.1               | 9.3    | 3.95  | 16.9  | 0.0222                | 72.9               |
|          | 512  | 45.8 ms          | 7.69 ms   | 8.64               | 6.52               | 7.38   | 3.61  | 12.2  | 0.00758               | 41.1               |
|          | 1024 | 96.3 ms          | 8.49 ms   | 5.98               | 4.48               | 4.99   | 2.38  | 8.65  | 0.00189               | 24.4               |
|          | 2048 | 396 ms           | 55 ms     | 4.18               | 3.07               | 3.54   | 1.8   | 5.94  | 0.00314               | 19.1               |
|          | 4096 | 1.88 s           | 51.9 ms   | 2.94               | 2.2                | 2.47   | 1.2   | 4.28  | 0.0114                | 14.4               |
|          | 8192 | 7.8 s            | 281 ms    | 2.08               | 1.56               | 1.73   | 0.839 | 2.95  | 0.00153               | 8.59               |

Table 5: **Simulation study.** Results for estimator `median1`. Mean, standard deviation, median,  $[0.25, 0.75]$  quantile, min and max of absolute error.

| $\kappa$ | $N$  | Computation time |           |                    |                    |         | Error   |        |                       |                    |
|----------|------|------------------|-----------|--------------------|--------------------|---------|---------|--------|-----------------------|--------------------|
|          |      | mean             | std. dev. | mean               | std. dev.          | median  | 0.25    | 0.75   | min                   | max                |
| 0        | 2    | 54.7 ms          | 9.84 ms   | 116                | 1050               | 0.926   | 0.341   | 2.88   | $3.33 \times 10^{-6}$ | $2.51 \times 10^4$ |
|          | 4    | 54.2 ms          | 8.33 ms   | 3.46               | 23.8               | 0.793   | 0.333   | 1.57   | 0.00578               | 503                |
|          | 8    | 53.5 ms          | 8.27 ms   | 0.767              | 0.925              | 0.522   | 0.232   | 0.977  | 0.00138               | 11.6               |
|          | 16   | 52.8 ms          | 8.6 ms    | 0.432              | 0.367              | 0.352   | 0.159   | 0.599  | $7.65 \times 10^{-4}$ | 2.28               |
|          | 32   | 52.7 ms          | 8.65 ms   | 0.263              | 0.209              | 0.22    | 0.1     | 0.39   | $1.77 \times 10^{-4}$ | 1.57               |
|          | 64   | 52.8 ms          | 9.24 ms   | 0.184              | 0.137              | 0.151   | 0.0757  | 0.266  | $1.24 \times 10^{-4}$ | 0.72               |
|          | 128  | 52.6 ms          | 8.45 ms   | 0.128              | 0.0949             | 0.112   | 0.0529  | 0.183  | $1.43 \times 10^{-4}$ | 0.624              |
|          | 256  | 59 ms            | 9.45 ms   | 0.0853             | 0.0667             | 0.0766  | 0.0312  | 0.124  | $1.37 \times 10^{-4}$ | 0.388              |
|          | 512  | 81.2 ms          | 9.95 ms   | 0.0609             | 0.0467             | 0.0541  | 0.0221  | 0.0924 | $7.51 \times 10^{-7}$ | 0.223              |
|          | 1024 | 172 ms           | 12 ms     | 0.0429             | 0.034              | 0.0367  | 0.0152  | 0.0622 | $1.73 \times 10^{-5}$ | 0.167              |
|          | 2048 | 574 ms           | 58.8 ms   | 0.0308             | 0.0243             | 0.0265  | 0.0103  | 0.0469 | $1.95 \times 10^{-5}$ | 0.125              |
|          | 4096 | 2.38 s           | 130 ms    | 0.0205             | 0.0166             | 0.0174  | 0.00571 | 0.032  | $8.49 \times 10^{-7}$ | 0.0702             |
| 0.01     | 8192 | 10.2 s           | 429 ms    | 0.0149             | 0.0124             | 0.0132  | 0.00327 | 0.023  | $2.94 \times 10^{-6}$ | 0.0618             |
|          | 2    | 53.4 ms          | 8 ms      | 4000               | $1.18 \times 10^5$ | 1.01    | 0.364   | 2.97   | $3.58 \times 10^{-4}$ | $3.73 \times 10^6$ |
|          | 4    | 52.4 ms          | 8.33 ms   | 7.13               | 123                | 0.799   | 0.338   | 1.68   | $1.81 \times 10^{-4}$ | 3720               |
|          | 8    | 52 ms            | 8.59 ms   | 0.799              | 1.25               | 0.548   | 0.211   | 0.976  | $1.17 \times 10^{-4}$ | 23.6               |
|          | 16   | 50.9 ms          | 8.17 ms   | 0.433              | 0.374              | 0.342   | 0.148   | 0.605  | $1.64 \times 10^{-4}$ | 3.15               |
|          | 32   | 51.3 ms          | 8.6 ms    | 0.273              | 0.224              | 0.226   | 0.105   | 0.383  | $5.62 \times 10^{-4}$ | 1.39               |
|          | 64   | 50.6 ms          | 8.66 ms   | 0.177              | 0.14               | 0.15    | 0.0623  | 0.26   | $1.18 \times 10^{-4}$ | 0.803              |
|          | 128  | 51.7 ms          | 9.14 ms   | 0.119              | 0.104              | 0.095   | 0.0323  | 0.177  | $1.25 \times 10^{-4}$ | 0.533              |
|          | 256  | 56.5 ms          | 9.12 ms   | 0.0759             | 0.0657             | 0.0628  | 0.0197  | 0.113  | $1.61 \times 10^{-5}$ | 0.4                |
|          | 512  | 77.2 ms          | 9.1 ms    | 0.055              | 0.0461             | 0.0461  | 0.0127  | 0.0845 | $4.21 \times 10^{-5}$ | 0.211              |
|          | 1024 | 155 ms           | 9.82 ms   | 0.0362             | 0.0331             | 0.0257  | 0.008   | 0.0578 | $1.14 \times 10^{-6}$ | 0.172              |
|          | 2048 | 553 ms           | 55 ms     | 0.0237             | 0.0212             | 0.0154  | 0.00792 | 0.0365 | $9.28 \times 10^{-6}$ | 0.103              |
| 0.1      | 4096 | 2.07 s           | 162 ms    | 0.016              | 0.0139             | 0.00986 | 0.00652 | 0.0235 | $6.45 \times 10^{-5}$ | 0.0672             |
|          | 8192 | 10 s             | 299 ms    | 0.0115             | 0.00885            | 0.00943 | 0.00551 | 0.0152 | $1.71 \times 10^{-5}$ | 0.052              |
|          | 2    | 53.5 ms          | 10 ms     | 441                | $1.02 \times 10^4$ | 1.05    | 0.34    | 3.38   | 0.00223               | $3.19 \times 10^5$ |
|          | 4    | 52.3 ms          | 8.42 ms   | 4.14               | 51.5               | 0.776   | 0.269   | 1.59   | $3.25 \times 10^{-4}$ | 1550               |
|          | 8    | 51.9 ms          | 8.3 ms    | 0.701              | 0.961              | 0.445   | 0.162   | 0.875  | $2.19 \times 10^{-4}$ | 10.4               |
|          | 16   | 51.5 ms          | 8.72 ms   | 0.374              | 0.408              | 0.267   | 0.0801  | 0.549  | $1.59 \times 10^{-4}$ | 3.98               |
|          | 32   | 51.3 ms          | 8.96 ms   | 0.221              | 0.219              | 0.134   | 0.0623  | 0.329  | $2.9 \times 10^{-5}$  | 1.37               |
|          | 64   | 50.4 ms          | 8.63 ms   | 0.135              | 0.123              | 0.0913  | 0.0486  | 0.192  | $2.36 \times 10^{-4}$ | 0.751              |
|          | 128  | 51.6 ms          | 9.23 ms   | 0.0897             | 0.0777             | 0.0737  | 0.0342  | 0.112  | $3.15 \times 10^{-4}$ | 0.514              |
|          | 256  | 57.7 ms          | 9.51 ms   | 0.0711             | 0.0514             | 0.0651  | 0.0349  | 0.0953 | $1.18 \times 10^{-4}$ | 0.33               |
|          | 512  | 78.6 ms          | 9.06 ms   | 0.0595             | 0.038              | 0.0581  | 0.0271  | 0.0891 | $2.45 \times 10^{-4}$ | 0.194              |
|          | 1024 | 186 ms           | 13.1 ms   | 0.054              | 0.035              | 0.0507  | 0.0231  | 0.0919 | $3.41 \times 10^{-4}$ | 0.177              |
| 1        | 2048 | 563 ms           | 56.3 ms   | 0.0499             | 0.0362             | 0.0397  | 0.0169  | 0.0945 | $3.53 \times 10^{-5}$ | 0.122              |
|          | 4096 | 2.03 s           | 178 ms    | 0.0439             | 0.0379             | 0.0268  | 0.0121  | 0.0968 | $6.28 \times 10^{-5}$ | 0.1                |
|          | 8192 | 9.95 s           | 265 ms    | 0.0402             | 0.0399             | 0.0192  | 0.00891 | 0.0985 | $2.38 \times 10^{-6}$ | 0.1                |
|          | 2    | 56.5 ms          | 8.71 ms   | $2.63 \times 10^4$ | $7.46 \times 10^5$ | 0.877   | 0.461   | 4.99   | 0.00623               | $2.35 \times 10^7$ |
|          | 4    | 55.5 ms          | 8.86 ms   | 7.32               | 45.9               | 0.776   | 0.357   | 2.41   | $2.96 \times 10^{-4}$ | 1190               |
|          | 8    | 54.5 ms          | 8.79 ms   | 1.23               | 3.35               | 0.588   | 0.251   | 1.09   | $1.52 \times 10^{-4}$ | 65                 |
|          | 16   | 54.2 ms          | 8.7 ms    | 0.632              | 0.712              | 0.442   | 0.208   | 0.827  | 0.00101               | 6.2                |
|          | 32   | 54.2 ms          | 8.83 ms   | 0.387              | 0.356              | 0.28    | 0.135   | 0.528  | $2.24 \times 10^{-4}$ | 2.93               |
|          | 64   | 54.6 ms          | 8.96 ms   | 0.292              | 0.271              | 0.206   | 0.101   | 0.376  | $2.36 \times 10^{-5}$ | 1.73               |
|          | 128  | 56 ms            | 9.03 ms   | 0.214              | 0.241              | 0.143   | 0.0624  | 0.266  | $2.1 \times 10^{-5}$  | 1                  |
|          | 256  | 61.6 ms          | 9.63 ms   | 0.176              | 0.244              | 0.106   | 0.0497  | 0.182  | $1.39 \times 10^{-5}$ | 1                  |
|          | 512  | 81 ms            | 9.47 ms   | 0.121              | 0.206              | 0.0654  | 0.03    | 0.121  | $2 \times 10^{-5}$    | 1                  |
| 10       | 1024 | 160 ms           | 10.3 ms   | 0.106              | 0.216              | 0.0514  | 0.0256  | 0.087  | $8.36 \times 10^{-6}$ | 1                  |
|          | 2048 | 573 ms           | 55.7 ms   | 0.114              | 0.26               | 0.0355  | 0.0177  | 0.065  | $3.91 \times 10^{-5}$ | 1                  |
|          | 4096 | 2.38 s           | 231 ms    | 0.0788             | 0.221              | 0.0239  | 0.0113  | 0.0423 | $4.2 \times 10^{-5}$  | 1                  |
|          | 8192 | 10 s             | 487 ms    | 0.0743             | 0.226              | 0.0177  | 0.00822 | 0.03   | $1.68 \times 10^{-5}$ | 1                  |
|          | 2    | 62 ms            | 10.9 ms   | $2.65 \times 10^4$ | $7.44 \times 10^5$ | 9.85    | 5.02    | 85.1   | 0.0101                | $2.35 \times 10^7$ |
|          | 4    | 61.2 ms          | 10.6 ms   | 191                | 2940               | 8.25    | 3.6     | 39.2   | 0.00318               | $9.18 \times 10^4$ |
|          | 8    | 59.7 ms          | 9.67 ms   | 16.2               | 38.1               | 5.21    | 2.45    | 14.6   | 0.00622               | 575                |
|          | 16   | 59.9 ms          | 10.2 ms   | 7.64               | 12.7               | 3.72    | 1.74    | 7.47   | 0.00722               | 196                |
|          | 32   | 60.1 ms          | 10.6 ms   | 4.02               | 4.53               | 2.78    | 1.38    | 4.72   | 0.00204               | 37.6               |
|          | 64   | 60.3 ms          | 10.2 ms   | 2.56               | 2.35               | 2.07    | 0.968   | 3.26   | 0.00184               | 21                 |
|          | 128  | 60 ms            | 10.3 ms   | 1.68               | 1.46               | 1.3     | 0.623   | 2.3    | $2.46 \times 10^{-4}$ | 10.6               |
|          | 256  | 66.3 ms          | 10.7 ms   | 1.14               | 0.973              | 0.938   | 0.392   | 1.63   | $1.53 \times 10^{-4}$ | 7.07               |
| 100      | 512  | 84.7 ms          | 11.2 ms   | 0.783              | 0.615              | 0.653   | 0.306   | 1.11   | $3.73 \times 10^{-4}$ | 3.63               |
|          | 1024 | 169 ms           | 16 ms     | 0.552              | 0.428              | 0.467   | 0.211   | 0.787  | $9.16 \times 10^{-5}$ | 2.48               |
|          | 2048 | 516 ms           | 76 ms     | 0.396              | 0.307              | 0.328   | 0.162   | 0.553  | 0.00253               | 2.02               |
|          | 4096 | 2.26 s           | 106 ms    | 0.287              | 0.215              | 0.244   | 0.114   | 0.427  | $2.23 \times 10^{-4}$ | 1.29               |
|          | 8192 | 9.96 s           | 819 ms    | 0.198              | 0.152              | 0.166   | 0.0775  | 0.276  | $3.86 \times 10^{-5}$ | 0.781              |
|          | 2    | 57.6 ms          | 8.69 ms   | $3.7 \times 10^4$  | $6.06 \times 10^5$ | 84.4    | 47      | 606    | 0.108                 | $1.79 \times 10^7$ |
|          | 4    | 58.5 ms          | 9.46 ms   | 4970               | $1.11 \times 10^5$ | 75.5    | 35.9    | 327    | 0.421                 | $3.32 \times 10^6$ |
|          | 8    | 57.1 ms          | 9.12 ms   | 150                | 374                | 52.4    | 26      | 134    | 0.0228                | 5310               |
|          | 16   | 57 ms            | 9.41 ms   | 68.5               | 98.1               | 38.1    | 18.4    | 72.4   | 0.0747                | 996                |
|          | 32   | 56.9 ms          | 9.24 ms   | 41.5               | 45.7               | 27.6    | 13.3    | 51.1   | 0.0374                | 478                |
|          | 64   | 56.7 ms          | 9.76 ms   | 25.9               | 25.2               | 19.6    | 9.25    | 34     | 0.13                  | 268                |
|          | 128  | 57.4 ms          | 9.25 ms   | 17.4               | 14.9               | 13.8    | 6.93    | 23.6   | 0.00296               | 115                |
|          | 256  | 61.5 ms          | 9.82 ms   | 11.8               | 10.1               | 9.27    | 4.01    | 16.8   | 0.00661               | 73.1               |
|          | 512  | 77.6 ms          | 9.78 ms   | 8.64               | 6.55               | 7.37    | 3.68    | 12.3   | 0.0234                | 41.3               |
|          | 1024 | 152 ms           | 15.6 ms   | 5.99               | 4.49               | 5.05    | 2.33    | 8.65   | 0.0428                | 24.7               |
|          | 2048 | 552 ms           | 20.4 ms   | 4.18               | 3.08               | 3.58    | 1.77    | 5.86   | $5.94 \times 10^{-4}$ | 19.3               |
|          | 4096 | 2.11 s           | 95.6 ms   | 2.93               | 2.21               | 2.44    | 1.18    | 4.2    | $7.25 \times 10^{-4}$ | 14.6               |
|          | 8192 | 8.68 s           | 677 ms    | 2.07               | 1.57               | 1.73    | 0.85    | 2.96   | 0.00869               | 8.34               |

Table 6: **Simulation study.** Results for estimator `median2`. Mean, standard deviation, median, [0.25, 0.75] quantile, min and max of absolute error.

| $\kappa$ | $N$  | Computation time |          | Error |           |        |        |       |                       |       |
|----------|------|------------------|----------|-------|-----------|--------|--------|-------|-----------------------|-------|
|          |      | mean             | std. dev | mean  | std. dev. | median | 0.25   | 0.75  | min                   | max   |
| 0        | 2    | 26.3 ms          | 6.21 ms  | N/A   | N/A       | N/A    | N/A    | N/A   | N/A                   | N/A   |
|          | 4    | 26.5 ms          | 6.27 ms  | 0.252 | 0.711     | 0.141  | 0.103  | 0.221 | 0.0374                | 17.6  |
|          | 8    | 26.7 ms          | 6.23 ms  | 0.333 | 0.146     | 0.294  | 0.247  | 0.373 | 0.135                 | 1.35  |
|          | 16   | 26.1 ms          | 6.08 ms  | 0.345 | 0.08      | 0.33   | 0.29   | 0.381 | 0.213                 | 0.86  |
|          | 32   | 26.5 ms          | 6.31 ms  | 0.335 | 0.0485    | 0.328  | 0.301  | 0.361 | 0.227                 | 0.575 |
|          | 64   | 26.3 ms          | 6.35 ms  | 0.326 | 0.0347    | 0.323  | 0.3    | 0.348 | 0.25                  | 0.513 |
|          | 128  | 26.5 ms          | 6.2 ms   | 0.318 | 0.0241    | 0.317  | 0.3    | 0.332 | 0.256                 | 0.398 |
|          | 256  | 26.6 ms          | 6.19 ms  | 0.312 | 0.0167    | 0.311  | 0.3    | 0.323 | 0.266                 | 0.375 |
|          | 512  | 26.2 ms          | 6.24 ms  | 0.309 | 0.0113    | 0.308  | 0.301  | 0.316 | 0.281                 | 0.346 |
|          | 1024 | 26.5 ms          | 6.21 ms  | 0.306 | 0.00854   | 0.306  | 0.3    | 0.312 | 0.283                 | 0.337 |
|          | 2048 | 26.8 ms          | 6.4 ms   | 0.306 | 0.00624   | 0.305  | 0.301  | 0.31  | 0.287                 | 0.324 |
|          | 4096 | 26.6 ms          | 6.32 ms  | 0.305 | 0.00436   | 0.305  | 0.302  | 0.308 | 0.291                 | 0.319 |
|          | 8192 | 27.9 ms          | 6.57 ms  | 0.305 | 0.00302   | 0.305  | 0.302  | 0.307 | 0.295                 | 0.316 |
| 0.01     | 2    | 22.8 ms          | 5.33 ms  | N/A   | N/A       | N/A    | N/A    | N/A   | N/A                   | N/A   |
|          | 4    | 23 ms            | 5.12 ms  | 0.186 | 0.328     | 0.115  | 0.0798 | 0.184 | 0.0277                | 5.93  |
|          | 8    | 23.2 ms          | 5.35 ms  | 0.311 | 0.132     | 0.278  | 0.228  | 0.359 | 0.123                 | 1.41  |
|          | 16   | 23.5 ms          | 5.55 ms  | 0.337 | 0.0778    | 0.322  | 0.285  | 0.368 | 0.191                 | 0.824 |
|          | 32   | 23.1 ms          | 5.26 ms  | 0.328 | 0.0529    | 0.32   | 0.29   | 0.357 | 0.22                  | 0.657 |
|          | 64   | 22.7 ms          | 5.07 ms  | 0.317 | 0.0345    | 0.316  | 0.292  | 0.339 | 0.23                  | 0.433 |
|          | 128  | 23 ms            | 5.28 ms  | 0.31  | 0.0249    | 0.308  | 0.293  | 0.324 | 0.243                 | 0.422 |
|          | 256  | 22.9 ms          | 5 ms     | 0.303 | 0.0172    | 0.302  | 0.292  | 0.315 | 0.251                 | 0.361 |
|          | 512  | 23.2 ms          | 5.25 ms  | 0.299 | 0.0115    | 0.299  | 0.292  | 0.306 | 0.267                 | 0.337 |
|          | 1024 | 23.1 ms          | 5.15 ms  | 0.297 | 0.00859   | 0.297  | 0.291  | 0.303 | 0.272                 | 0.329 |
|          | 2048 | 23.2 ms          | 5.06 ms  | 0.295 | 0.00611   | 0.295  | 0.291  | 0.3   | 0.274                 | 0.313 |
|          | 4096 | 23.8 ms          | 5.44 ms  | 0.295 | 0.00438   | 0.295  | 0.292  | 0.298 | 0.283                 | 0.308 |
|          | 8192 | 24.6 ms          | 5.57 ms  | 0.294 | 0.0033    | 0.294  | 0.292  | 0.297 | 0.284                 | 0.305 |
| 0.1      | 2    | 23 ms            | 5.63 ms  | N/A   | N/A       | N/A    | N/A    | N/A   | N/A                   | N/A   |
|          | 4    | 23 ms            | 5.21 ms  | 0.126 | 0.373     | 0.0498 | 0.0269 | 0.112 | $9.77 \times 10^{-6}$ | 9.38  |
|          | 8    | 23.4 ms          | 5.53 ms  | 0.227 | 0.146     | 0.188  | 0.138  | 0.261 | 0.0454                | 1.31  |
|          | 16   | 23.2 ms          | 5.06 ms  | 0.253 | 0.0902    | 0.236  | 0.192  | 0.289 | 0.109                 | 0.882 |
|          | 32   | 23.3 ms          | 5.34 ms  | 0.244 | 0.0565    | 0.237  | 0.204  | 0.274 | 0.124                 | 0.588 |
|          | 64   | 22.8 ms          | 5.04 ms  | 0.231 | 0.0376    | 0.226  | 0.205  | 0.253 | 0.138                 | 0.412 |
|          | 128  | 23.3 ms          | 5.55 ms  | 0.222 | 0.0272    | 0.221  | 0.203  | 0.238 | 0.155                 | 0.334 |
|          | 256  | 23 ms            | 5.13 ms  | 0.219 | 0.0219    | 0.218  | 0.203  | 0.234 | 0.162                 | 0.298 |
|          | 512  | 23.1 ms          | 5.32 ms  | 0.215 | 0.0175    | 0.216  | 0.202  | 0.227 | 0.165                 | 0.265 |
|          | 1024 | 23.5 ms          | 5.31 ms  | 0.212 | 0.0152    | 0.213  | 0.201  | 0.223 | 0.167                 | 0.258 |
|          | 2048 | 23.6 ms          | 5.35 ms  | 0.212 | 0.0139    | 0.215  | 0.201  | 0.223 | 0.175                 | 0.249 |
|          | 4096 | 23.8 ms          | 5.31 ms  | 0.213 | 0.0125    | 0.216  | 0.205  | 0.222 | 0.181                 | 0.235 |
|          | 8192 | 24.5 ms          | 5.5 ms   | 0.213 | 0.0121    | 0.216  | 0.205  | 0.222 | 0.183                 | 0.232 |
| 1        | 2    | 23.3 ms          | 5.44 ms  | N/A   | N/A       | N/A    | N/A    | N/A   | N/A                   | N/A   |
|          | 4    | 23.6 ms          | 5.27 ms  | 0.92  | 1.44      | 0.846  | 0.707  | 0.939 | 0.00372               | 29.8  |
|          | 8    | 23.8 ms          | 5.36 ms  | 0.57  | 0.343     | 0.6    | 0.42   | 0.723 | 0.00163               | 6.34  |
|          | 16   | 23.9 ms          | 5.57 ms  | 0.438 | 0.184     | 0.473  | 0.319  | 0.575 | $2.52 \times 10^{-4}$ | 1.47  |
|          | 32   | 23.5 ms          | 5.25 ms  | 0.398 | 0.153     | 0.419  | 0.304  | 0.51  | $7.46 \times 10^{-5}$ | 0.769 |
|          | 64   | 23.5 ms          | 5.32 ms  | 0.395 | 0.119     | 0.406  | 0.326  | 0.478 | 0.00628               | 0.722 |
|          | 128  | 23.7 ms          | 5.41 ms  | 0.397 | 0.0876    | 0.402  | 0.34   | 0.455 | 0.0628                | 0.759 |
|          | 256  | 23.3 ms          | 5.15 ms  | 0.399 | 0.065     | 0.398  | 0.357  | 0.442 | 0.182                 | 0.61  |
|          | 512  | 23.7 ms          | 5.45 ms  | 0.399 | 0.0507    | 0.396  | 0.364  | 0.43  | 0.229                 | 0.605 |
|          | 1024 | 23.6 ms          | 5.42 ms  | 0.395 | 0.0387    | 0.392  | 0.369  | 0.415 | 0.293                 | 0.573 |
|          | 2048 | 23.8 ms          | 5.38 ms  | 0.393 | 0.032     | 0.389  | 0.372  | 0.409 | 0.313                 | 0.554 |
|          | 4096 | 24.2 ms          | 5.36 ms  | 0.392 | 0.0263    | 0.388  | 0.376  | 0.402 | 0.333                 | 0.546 |
|          | 8192 | 24.8 ms          | 5.4 ms   | 0.391 | 0.0224    | 0.386  | 0.377  | 0.4   | 0.343                 | 0.544 |
| 10       | 2    | 22.4 ms          | 5.13 ms  | N/A   | N/A       | N/A    | N/A    | N/A   | N/A                   | N/A   |
|          | 4    | 23 ms            | 5.17 ms  | 9.25  | 11.4      | 8.76   | 6.28   | 9.96  | 0.0177                | 244   |
|          | 8    | 22.7 ms          | 4.91 ms  | 6.73  | 4.87      | 6.27   | 3.23   | 9.83  | 0.0217                | 52.7  |
|          | 16   | 23.2 ms          | 5.2 ms   | 5.56  | 3.75      | 4.52   | 2.28   | 9.58  | 0.00478               | 23.6  |
|          | 32   | 23 ms            | 5.11 ms  | 4.52  | 3.58      | 2.94   | 1.4    | 9.1   | 0.00622               | 10.3  |
|          | 64   | 23.2 ms          | 5.09 ms  | 3.7   | 3.33      | 2.04   | 0.941  | 8.25  | 0.0156                | 8.46  |
|          | 128  | 23.2 ms          | 5.03 ms  | 2.88  | 2.82      | 1.48   | 0.656  | 6.9   | $7.33 \times 10^{-4}$ | 7.31  |
|          | 256  | 23.2 ms          | 5.15 ms  | 2.15  | 2.14      | 1.09   | 0.473  | 5.12  | 0.00307               | 5.91  |
|          | 512  | 23.1 ms          | 5.06 ms  | 1.52  | 1.41      | 0.873  | 0.438  | 3.34  | $3.26 \times 10^{-4}$ | 4.53  |
|          | 1024 | 22.9 ms          | 4.92 ms  | 1.09  | 0.874     | 0.762  | 0.391  | 2.08  | 0.00333               | 3.17  |
|          | 2048 | 23.5 ms          | 5.35 ms  | 0.791 | 0.488     | 0.686  | 0.42   | 1.14  | 0.012                 | 2.08  |
|          | 4096 | 23.7 ms          | 5.24 ms  | 0.658 | 0.291     | 0.628  | 0.447  | 0.847 | 0.00161               | 1.54  |
|          | 8192 | 24.1 ms          | 5.39 ms  | 0.584 | 0.178     | 0.575  | 0.456  | 0.703 | 0.0804                | 1.21  |
| 100      | 2    | 23.7 ms          | 5.82 ms  | N/A   | N/A       | N/A    | N/A    | N/A   | N/A                   | N/A   |
|          | 4    | 23.9 ms          | 5.48 ms  | 91.3  | 171       | 100    | 67.3   | 100   | 0.0532                | 5030  |
|          | 8    | 23.9 ms          | 5.67 ms  | 73.7  | 41.6      | 99.8   | 39.3   | 99.8  | $8.2 \times 10^{-4}$  | 450   |
|          | 16   | 23.6 ms          | 5.1 ms   | 64.1  | 39.1      | 99.6   | 25.7   | 99.6  | 0.0409                | 194   |
|          | 32   | 23.6 ms          | 5.24 ms  | 58.2  | 40.8      | 51.9   | 16.7   | 99.2  | 0.00166               | 114   |
|          | 64   | 23.5 ms          | 5.29 ms  | 53.6  | 42.4      | 32.4   | 12.2   | 98.3  | 0.0531                | 98.4  |
|          | 128  | 23.6 ms          | 5.24 ms  | 49.9  | 43.5      | 23.3   | 7.56   | 96.6  | 0.0217                | 96.7  |
|          | 256  | 23.4 ms          | 5.19 ms  | 46.6  | 43.1      | 15.8   | 5.68   | 93.4  | 0.0776                | 93.6  |
|          | 512  | 23.7 ms          | 5.36 ms  | 42.3  | 41.2      | 11     | 3.87   | 87.5  | 0.00602               | 87.8  |
|          | 1024 | 23.7 ms          | 5.46 ms  | 35.9  | 36.8      | 7.3    | 2.6    | 77.6  | $9.52 \times 10^{-4}$ | 78.2  |
|          | 2048 | 23.7 ms          | 5.25 ms  | 28.3  | 30.1      | 4.82   | 1.86   | 63.2  | 0.00521               | 64.5  |
|          | 4096 | 23.8 ms          | 5.31 ms  | 21.9  | 22.1      | 4.13   | 1.39   | 46.1  | $6.78 \times 10^{-4}$ | 47.8  |
|          | 8192 | 24.7 ms          | 5.63 ms  | 13.9  | 14.2      | 2.75   | 0.968  | 29.8  | 0.00235               | 32    |

Table 7: **Simulation study.** Results for estimator **linear**. Mean, standard deviation, median, [0.25, 0.75] quantile, min and max of absolute error.

| $\kappa$ | $N$  | Computation time |           | mean               | std. dev.          | median  | Error   |         |                       |                    |
|----------|------|------------------|-----------|--------------------|--------------------|---------|---------|---------|-----------------------|--------------------|
|          |      | mean             | std. dev. |                    |                    |         | 0.25    | 0.75    | min                   | max                |
| 0        | 2    | 24.3 ms          | 5.54 ms   | 0.273              | 0.166              | 0.274   | 0.12    | 0.427   | $6.69 \times 10^{-6}$ | 0.522              |
|          | 4    | 23.7 ms          | 5.44 ms   | 0.391              | 0.923              | 0.195   | 0.115   | 0.328   | 0.0029                | 18.9               |
|          | 8    | 24.2 ms          | 5.75 ms   | 0.258              | 0.296              | 0.157   | 0.0932  | 0.273   | 0.00578               | 2.57               |
|          | 16   | 24.2 ms          | 5.58 ms   | 0.183              | 0.194              | 0.112   | 0.0636  | 0.213   | 0.00366               | 1.26               |
|          | 32   | 24.1 ms          | 5.67 ms   | 0.133              | 0.138              | 0.0774  | 0.0443  | 0.156   | 0.00104               | 0.797              |
|          | 64   | 24 ms            | 5.51 ms   | 0.102              | 0.0998             | 0.0611  | 0.036   | 0.129   | 0.00115               | 0.699              |
|          | 128  | 24.1 ms          | 5.52 ms   | 0.0737             | 0.0737             | 0.0445  | 0.0246  | 0.0938  | 0.00105               | 0.406              |
|          | 256  | 24 ms            | 5.59 ms   | 0.0507             | 0.0531             | 0.0285  | 0.0164  | 0.0631  | 0.00113               | 0.293              |
|          | 512  | 24.2 ms          | 5.61 ms   | 0.0356             | 0.036              | 0.0212  | 0.0114  | 0.0473  | $6.5 \times 10^{-4}$  | 0.184              |
|          | 1024 | 23.9 ms          | 5.47 ms   | 0.0269             | 0.0272             | 0.0154  | 0.00864 | 0.0356  | $2.69 \times 10^{-4}$ | 0.151              |
|          | 2048 | 24 ms            | 5.59 ms   | 0.0198             | 0.0194             | 0.0119  | 0.00619 | 0.0262  | $4.74 \times 10^{-4}$ | 0.106              |
|          | 4096 | 24.4 ms          | 5.82 ms   | 0.0137             | 0.0137             | 0.00791 | 0.00434 | 0.019   | $1.84 \times 10^{-4}$ | 0.0801             |
|          | 8192 | 24.6 ms          | 5.8 ms    | 0.00962            | 0.00944            | 0.00574 | 0.00313 | 0.0128  | $8.8 \times 10^{-5}$  | 0.0562             |
| 0.01     | 2    | 24.3 ms          | 5.67 ms   | 0.269              | 0.165              | 0.269   | 0.117   | 0.419   | $9.77 \times 10^{-5}$ | 0.512              |
|          | 4    | 24.2 ms          | 5.6 ms    | 0.389              | 0.713              | 0.189   | 0.107   | 0.331   | $3.82 \times 10^{-4}$ | 7.55               |
|          | 8    | 23.7 ms          | 5.22 ms   | 0.246              | 0.283              | 0.144   | 0.079   | 0.296   | 0.00112               | 2.16               |
|          | 16   | 23.9 ms          | 5.48 ms   | 0.18               | 0.2                | 0.108   | 0.0574  | 0.216   | $8.42 \times 10^{-5}$ | 1.44               |
|          | 32   | 23.9 ms          | 5.49 ms   | 0.132              | 0.144              | 0.0755  | 0.0372  | 0.177   | $1.91 \times 10^{-4}$ | 1.06               |
|          | 64   | 24 ms            | 5.53 ms   | 0.0952             | 0.102              | 0.0534  | 0.0251  | 0.126   | $5.56 \times 10^{-5}$ | 0.53               |
|          | 128  | 24.1 ms          | 5.77 ms   | 0.0713             | 0.0831             | 0.0364  | 0.0144  | 0.0979  | $1.23 \times 10^{-4}$ | 0.475              |
|          | 256  | 24.2 ms          | 5.51 ms   | 0.046              | 0.0554             | 0.0212  | 0.0085  | 0.065   | $2.37 \times 10^{-6}$ | 0.276              |
|          | 512  | 24.1 ms          | 5.43 ms   | 0.0297             | 0.0372             | 0.012   | 0.00449 | 0.0408  | $4.25 \times 10^{-5}$ | 0.186              |
|          | 1024 | 24.2 ms          | 5.57 ms   | 0.0203             | 0.0268             | 0.00742 | 0.00335 | 0.0277  | $1.3 \times 10^{-5}$  | 0.135              |
|          | 2048 | 24.2 ms          | 5.66 ms   | 0.0138             | 0.0176             | 0.00639 | 0.00304 | 0.0167  | $6.32 \times 10^{-7}$ | 0.105              |
|          | 4096 | 24.4 ms          | 5.58 ms   | 0.0102             | 0.011              | 0.0063  | 0.00336 | 0.011   | $2.6 \times 10^{-5}$  | 0.0582             |
|          | 8192 | 24.2 ms          | 5.47 ms   | 0.00844            | 0.00713            | 0.00665 | 0.00417 | 0.00918 | $3.91 \times 10^{-5}$ | 0.0476             |
| 0.1      | 2    | 24.6 ms          | 5.8 ms    | 0.205              | 0.141              | 0.199   | 0.0674  | 0.34    | $2.52 \times 10^{-4}$ | 0.422              |
|          | 4    | 24.5 ms          | 5.88 ms   | 0.311              | 0.699              | 0.11    | 0.0474  | 0.242   | $1.18 \times 10^{-4}$ | 10.8               |
|          | 8    | 24.2 ms          | 5.78 ms   | 0.184              | 0.285              | 0.0672  | 0.0307  | 0.183   | $2.75 \times 10^{-4}$ | 1.89               |
|          | 16   | 24 ms            | 5.5 ms    | 0.145              | 0.206              | 0.0608  | 0.03    | 0.154   | $8.56 \times 10^{-5}$ | 1.36               |
|          | 32   | 24.2 ms          | 5.62 ms   | 0.109              | 0.13               | 0.0597  | 0.0342  | 0.122   | $1.21 \times 10^{-4}$ | 0.971              |
|          | 64   | 24.1 ms          | 5.61 ms   | 0.0862             | 0.0843             | 0.063   | 0.0381  | 0.0869  | $2.73 \times 10^{-4}$ | 0.534              |
|          | 128  | 24.2 ms          | 5.69 ms   | 0.0736             | 0.0542             | 0.0658  | 0.0433  | 0.0847  | $4.54 \times 10^{-4}$ | 0.375              |
|          | 256  | 24.2 ms          | 5.75 ms   | 0.0665             | 0.0387             | 0.0681  | 0.0407  | 0.0846  | $3.34 \times 10^{-6}$ | 0.282              |
|          | 512  | 24.1 ms          | 5.72 ms   | 0.0544             | 0.0332             | 0.0542  | 0.0257  | 0.0802  | $1.36 \times 10^{-4}$ | 0.208              |
|          | 1024 | 24.1 ms          | 5.62 ms   | 0.0399             | 0.0296             | 0.0338  | 0.0145  | 0.0617  | $2.48 \times 10^{-5}$ | 0.146              |
|          | 2048 | 24.2 ms          | 5.69 ms   | 0.0277             | 0.0218             | 0.0225  | 0.0104  | 0.0399  | $3.41 \times 10^{-5}$ | 0.102              |
|          | 4096 | 24.1 ms          | 5.53 ms   | 0.0182             | 0.0141             | 0.0146  | 0.00725 | 0.0263  | $6.76 \times 10^{-5}$ | 0.076              |
|          | 8192 | 24.5 ms          | 5.69 ms   | 0.0132             | 0.00969            | 0.0112  | 0.00533 | 0.0193  | $7.38 \times 10^{-6}$ | 0.0631             |
| 1        | 2    | 24.6 ms          | 6.06 ms   | $3.72 \times 10^5$ | $1.18 \times 10^7$ | 0.652   | 0.526   | 0.818   | 0.478                 | $3.72 \times 10^8$ |
|          | 4    | 24.5 ms          | 5.91 ms   | 1.05               | 2.09               | 0.755   | 0.549   | 0.87    | 0.00557               | 31.1               |
|          | 8    | 24 ms            | 5.62 ms   | 0.598              | 0.49               | 0.593   | 0.295   | 0.815   | $5.95 \times 10^{-4}$ | 7.07               |
|          | 16   | 23.8 ms          | 5.57 ms   | 0.415              | 0.293              | 0.359   | 0.181   | 0.606   | 0.001                 | 2.17               |
|          | 32   | 23.8 ms          | 5.57 ms   | 0.271              | 0.206              | 0.234   | 0.109   | 0.383   | $6.22 \times 10^{-4}$ | 1.29               |
|          | 64   | 23.9 ms          | 5.68 ms   | 0.178              | 0.138              | 0.15    | 0.0694  | 0.256   | $4.15 \times 10^{-4}$ | 0.848              |
|          | 128  | 24 ms            | 5.66 ms   | 0.122              | 0.0922             | 0.101   | 0.0522  | 0.175   | $2.67 \times 10^{-4}$ | 0.587              |
|          | 256  | 23.7 ms          | 5.52 ms   | 0.0843             | 0.0652             | 0.0693  | 0.033   | 0.123   | $1.25 \times 10^{-4}$ | 0.3                |
|          | 512  | 24 ms            | 5.74 ms   | 0.0598             | 0.0459             | 0.0483  | 0.0235  | 0.0873  | $8.31 \times 10^{-5}$ | 0.244              |
|          | 1024 | 23.9 ms          | 5.54 ms   | 0.0417             | 0.0321             | 0.0361  | 0.0159  | 0.0595  | $4.68 \times 10^{-5}$ | 0.17               |
|          | 2048 | 23.8 ms          | 5.35 ms   | 0.0305             | 0.0226             | 0.0262  | 0.0121  | 0.0441  | $5.19 \times 10^{-5}$ | 0.118              |
|          | 4096 | 24.2 ms          | 5.67 ms   | 0.0207             | 0.0158             | 0.0176  | 0.00791 | 0.0298  | $1.79 \times 10^{-5}$ | 0.0945             |
|          | 8192 | 24.3 ms          | 5.6 ms    | 0.0147             | 0.011              | 0.0124  | 0.00575 | 0.0212  | $1.72 \times 10^{-5}$ | 0.0636             |
| 10       | 2    | 25 ms            | 5.79 ms   | $1.99 \times 10^5$ | $6.3 \times 10^6$  | 9.49    | 9.48    | 9.52    | 9.48                  | $1.99 \times 10^8$ |
|          | 4    | 24.7 ms          | 5.96 ms   | 7.76               | 14.9               | 5.19    | 3.34    | 7.01    | 0.00459               | 245                |
|          | 8    | 24.1 ms          | 5.45 ms   | 4.67               | 6.22               | 3.49    | 1.89    | 5.15    | 0.00539               | 96.6               |
|          | 16   | 24.3 ms          | 5.65 ms   | 3.01               | 2.98               | 2.42    | 1.27    | 3.8     | 0.00795               | 42.2               |
|          | 32   | 24.2 ms          | 5.6 ms    | 1.97               | 1.6                | 1.66    | 0.813   | 2.74    | 0.00136               | 15                 |
|          | 64   | 24.3 ms          | 5.58 ms   | 1.38               | 1.13               | 1.14    | 0.513   | 1.99    | $9.76 \times 10^{-5}$ | 8.3                |
|          | 128  | 24.3 ms          | 5.81 ms   | 0.953              | 0.745              | 0.785   | 0.368   | 1.38    | 0.00238               | 4.65               |
|          | 256  | 24.3 ms          | 5.66 ms   | 0.668              | 0.518              | 0.574   | 0.269   | 0.961   | 0.00134               | 3.63               |
|          | 512  | 23.9 ms          | 5.29 ms   | 0.481              | 0.353              | 0.427   | 0.194   | 0.691   | $1.54 \times 10^{-4}$ | 1.89               |
|          | 1024 | 24.2 ms          | 5.67 ms   | 0.331              | 0.249              | 0.282   | 0.134   | 0.471   | $1.29 \times 10^{-4}$ | 1.34               |
|          | 2048 | 24.4 ms          | 5.56 ms   | 0.233              | 0.173              | 0.197   | 0.0974  | 0.334   | 0.00113               | 1.08               |
|          | 4096 | 24.8 ms          | 5.86 ms   | 0.163              | 0.122              | 0.138   | 0.0686  | 0.233   | $1.11 \times 10^{-4}$ | 0.709              |
|          | 8192 | 24.8 ms          | 5.7 ms    | 0.117              | 0.0878             | 0.0971  | 0.0492  | 0.172   | $3.87 \times 10^{-5}$ | 0.527              |
| 100      | 2    | 25.9 ms          | 5.93 ms   | $5.18 \times 10^4$ | $1.28 \times 10^6$ | 99.5    | 99.5    | 99.5    | 99.5                  | $3.84 \times 10^7$ |
|          | 4    | 25.6 ms          | 6.03 ms   | 82                 | 204                | 65.8    | 42.7    | 79.4    | 0.0543                | 5030               |
|          | 8    | 25.3 ms          | 5.8 ms    | 47.9               | 57.6               | 38.2    | 20.7    | 56.1    | 0.0915                | 942                |
|          | 16   | 25.3 ms          | 5.79 ms   | 30.6               | 27.6               | 25.1    | 13      | 41.2    | 0.0041                | 339                |
|          | 32   | 24.9 ms          | 5.53 ms   | 21.4               | 18                 | 17.4    | 8.69    | 28.5    | 0.0265                | 129                |
|          | 64   | 24.8 ms          | 5.43 ms   | 14.7               | 11.6               | 12.5    | 5.92    | 20.9    | $9.16 \times 10^{-4}$ | 91.7               |
|          | 128  | 25.4 ms          | 6.18 ms   | 10.1               | 8.11               | 8.26    | 3.86    | 14.3    | 0.0121                | 51.9               |
|          | 256  | 25.4 ms          | 5.9 ms    | 7.2                | 5.61               | 6.14    | 2.85    | 10.3    | 0.00275               | 47                 |
|          | 512  | 25.3 ms          | 5.88 ms   | 4.96               | 3.88               | 4.31    | 1.77    | 7.3     | 0.0127                | 27                 |
|          | 1024 | 24.9 ms          | 5.61 ms   | 3.43               | 2.59               | 2.91    | 1.37    | 4.83    | 0.0198                | 14.2               |
|          | 2048 | 25.2 ms          | 5.74 ms   | 2.55               | 1.86               | 2.17    | 1.07    | 3.66    | $7.37 \times 10^{-4}$ | 10.6               |
|          | 4096 | 25.4 ms          | 5.82 ms   | 1.83               | 1.41               | 1.47    | 0.742   | 2.65    | 0.00109               | 8.48               |
|          | 8192 | 25.5 ms          | 5.76 ms   | 1.28               | 1.01               | 1.05    | 0.494   | 1.82    | 0.00355               | 5.87               |

Table 8: **Simulation study.** Results for estimator MML-2. Mean, standard deviation, median, [0.25, 0.75] quantile, min and max of absolute error.

| $\kappa$ | $N$  | Computation time |          | Error              |                    |        | 0.25    | 0.75   | min                   | max                |
|----------|------|------------------|----------|--------------------|--------------------|--------|---------|--------|-----------------------|--------------------|
|          |      | mean             | std. dev | mean               | std. dev.          | median |         |        |                       |                    |
| 0        | 2    | 23 ms            | 4.45 ms  | 0.501              | 0.33               | 0.471  | 0.203   | 0.781  | $6.69 \times 10^{-6}$ | 1.07               |
|          | 4    | 22.5 ms          | 4.27 ms  | 0.629              | 0.946              | 0.426  | 0.256   | 0.673  | 0.00665               | 18.9               |
|          | 8    | 22.7 ms          | 4.22 ms  | 0.472              | 0.32               | 0.404  | 0.258   | 0.585  | 0.0167                | 2.65               |
|          | 16   | 22.6 ms          | 4.3 ms   | 0.358              | 0.212              | 0.325  | 0.205   | 0.466  | 0.0125                | 1.33               |
|          | 32   | 22.7 ms          | 4.45 ms  | 0.269              | 0.15               | 0.244  | 0.157   | 0.352  | 0.004                 | 0.855              |
|          | 64   | 22.6 ms          | 4.31 ms  | 0.209              | 0.106              | 0.195  | 0.132   | 0.272  | 0.00473               | 0.733              |
|          | 128  | 22.5 ms          | 4.28 ms  | 0.152              | 0.0774             | 0.144  | 0.0934  | 0.198  | 0.00451               | 0.44               |
|          | 256  | 22.4 ms          | 4.11 ms  | 0.105              | 0.0568             | 0.0969 | 0.0636  | 0.139  | 0.00462               | 0.318              |
|          | 512  | 22.3 ms          | 3.86 ms  | 0.075              | 0.0392             | 0.0711 | 0.0451  | 0.101  | 0.00281               | 0.204              |
|          | 1024 | 22.3 ms          | 3.98 ms  | 0.055              | 0.0286             | 0.0515 | 0.0338  | 0.0727 | 0.00108               | 0.164              |
|          | 2048 | 22.4 ms          | 4.04 ms  | 0.0399             | 0.0203             | 0.0384 | 0.0243  | 0.0522 | 0.0019                | 0.115              |
|          | 4096 | 22.6 ms          | 4.19 ms  | 0.028              | 0.0143             | 0.0262 | 0.017   | 0.0372 | $2.2 \times 10^{-4}$  | 0.0861             |
|          | 8192 | 22.9 ms          | 4.35 ms  | 0.0198             | 0.00995            | 0.0188 | 0.0121  | 0.0259 | $2.87 \times 10^{-4}$ | 0.0604             |
| 0.01     | 2    | 24.3 ms          | 5.61 ms  | 0.504              | 0.33               | 0.47   | 0.206   | 0.776  | $6.23 \times 10^{-4}$ | 1.06               |
|          | 4    | 24 ms            | 5.81 ms  | 0.629              | 0.751              | 0.424  | 0.253   | 0.686  | $4.68 \times 10^{-4}$ | 7.65               |
|          | 8    | 23.9 ms          | 5.6 ms   | 0.458              | 0.314              | 0.388  | 0.237   | 0.612  | 0.00692               | 2.25               |
|          | 16   | 24.2 ms          | 5.69 ms  | 0.358              | 0.214              | 0.327  | 0.206   | 0.468  | 0.00115               | 1.5                |
|          | 32   | 24.1 ms          | 5.81 ms  | 0.271              | 0.152              | 0.251  | 0.156   | 0.366  | 0.00147               | 1.1                |
|          | 64   | 23.7 ms          | 5.43 ms  | 0.202              | 0.107              | 0.189  | 0.119   | 0.266  | 0.00507               | 0.577              |
|          | 128  | 23.8 ms          | 5.48 ms  | 0.147              | 0.0849             | 0.137  | 0.0829  | 0.196  | $2 \times 10^{-4}$    | 0.502              |
|          | 256  | 23.8 ms          | 5.72 ms  | 0.101              | 0.0573             | 0.0924 | 0.0604  | 0.137  | $1.31 \times 10^{-4}$ | 0.301              |
|          | 512  | 23.8 ms          | 5.47 ms  | 0.0681             | 0.0399             | 0.0628 | 0.0387  | 0.0929 | $5.83 \times 10^{-4}$ | 0.205              |
|          | 1024 | 23.8 ms          | 5.46 ms  | 0.0463             | 0.0291             | 0.0431 | 0.0237  | 0.064  | $3.03 \times 10^{-5}$ | 0.148              |
|          | 2048 | 23.7 ms          | 5.36 ms  | 0.0301             | 0.0205             | 0.0275 | 0.0137  | 0.0424 | $3.62 \times 10^{-5}$ | 0.113              |
|          | 4096 | 23.9 ms          | 5.54 ms  | 0.0193             | 0.0139             | 0.0173 | 0.00745 | 0.0284 | $3.25 \times 10^{-5}$ | 0.0651             |
|          | 8192 | 24.2 ms          | 5.74 ms  | 0.0128             | 0.00962            | 0.0107 | 0.00487 | 0.019  | $2.9 \times 10^{-5}$  | 0.0517             |
| 0.1      | 2    | 24.7 ms          | 5.76 ms  | 0.44               | 0.31               | 0.419  | 0.148   | 0.713  | 0.00107               | 0.972              |
|          | 4    | 24.1 ms          | 5.61 ms  | 0.548              | 0.736              | 0.356  | 0.185   | 0.598  | $1.11 \times 10^{-4}$ | 10.9               |
|          | 8    | 24.1 ms          | 5.72 ms  | 0.373              | 0.322              | 0.287  | 0.151   | 0.497  | $1.94 \times 10^{-4}$ | 1.99               |
|          | 16   | 24 ms            | 5.49 ms  | 0.293              | 0.228              | 0.252  | 0.117   | 0.401  | $5.94 \times 10^{-4}$ | 1.42               |
|          | 32   | 24.4 ms          | 6.05 ms  | 0.204              | 0.156              | 0.179  | 0.0742  | 0.299  | $7.64 \times 10^{-6}$ | 1.01               |
|          | 64   | 23.8 ms          | 5.54 ms  | 0.134              | 0.108              | 0.11   | 0.0466  | 0.193  | $6.84 \times 10^{-5}$ | 0.573              |
|          | 128  | 23.7 ms          | 5.42 ms  | 0.0883             | 0.0734             | 0.0691 | 0.0318  | 0.125  | $4.3 \times 10^{-5}$  | 0.403              |
|          | 256  | 23.4 ms          | 5.29 ms  | 0.0638             | 0.0517             | 0.0523 | 0.0238  | 0.0903 | $4.03 \times 10^{-5}$ | 0.3                |
|          | 512  | 23.9 ms          | 5.55 ms  | 0.047              | 0.0363             | 0.0403 | 0.0179  | 0.0677 | $3.79 \times 10^{-5}$ | 0.22               |
|          | 1024 | 23.9 ms          | 5.5 ms   | 0.034              | 0.0259             | 0.0286 | 0.0146  | 0.0481 | $8.8 \times 10^{-5}$  | 0.153              |
|          | 2048 | 23.8 ms          | 5.4 ms   | 0.0248             | 0.019              | 0.021  | 0.00951 | 0.0359 | $5.81 \times 10^{-6}$ | 0.107              |
|          | 4096 | 24.3 ms          | 5.59 ms  | 0.0174             | 0.0132             | 0.0145 | 0.00707 | 0.0256 | $2.81 \times 10^{-6}$ | 0.0676             |
|          | 8192 | 24.3 ms          | 5.52 ms  | 0.0131             | 0.00949            | 0.0115 | 0.00564 | 0.0192 | $2.73 \times 10^{-5}$ | 0.0568             |
| 1        | 2    | 25 ms            | 5.74 ms  | $3.79 \times 10^5$ | $1.2 \times 10^7$  | 0.389  | 0.0971  | 0.69   | $7.93 \times 10^{-4}$ | $3.79 \times 10^8$ |
|          | 4    | 24.5 ms          | 5.51 ms  | 0.922              | 2.13               | 0.538  | 0.293   | 0.775  | $5.39 \times 10^{-4}$ | 31.1               |
|          | 8    | 24.5 ms          | 5.46 ms  | 0.465              | 0.506              | 0.363  | 0.177   | 0.619  | $2.04 \times 10^{-4}$ | 7.1                |
|          | 16   | 24.1 ms          | 5.26 ms  | 0.341              | 0.268              | 0.291  | 0.136   | 0.482  | $3.93 \times 10^{-4}$ | 2.2                |
|          | 32   | 24.1 ms          | 5.1 ms   | 0.243              | 0.19               | 0.209  | 0.0979  | 0.341  | $2.52 \times 10^{-4}$ | 1.3                |
|          | 64   | 24.3 ms          | 5.53 ms  | 0.17               | 0.133              | 0.146  | 0.062   | 0.241  | $9.5 \times 10^{-5}$  | 0.859              |
|          | 128  | 24 ms            | 5.24 ms  | 0.119              | 0.0906             | 0.101  | 0.0469  | 0.172  | $3.39 \times 10^{-4}$ | 0.593              |
|          | 256  | 24.3 ms          | 5.5 ms   | 0.0834             | 0.0646             | 0.067  | 0.0315  | 0.121  | $6.53 \times 10^{-5}$ | 0.304              |
|          | 512  | 24.1 ms          | 5.29 ms  | 0.0594             | 0.0458             | 0.0483 | 0.0229  | 0.0864 | $7.49 \times 10^{-5}$ | 0.246              |
|          | 1024 | 24.3 ms          | 5.54 ms  | 0.0416             | 0.032              | 0.0362 | 0.0161  | 0.0597 | $1.16 \times 10^{-4}$ | 0.171              |
|          | 2048 | 24.3 ms          | 5.49 ms  | 0.0305             | 0.0226             | 0.0262 | 0.012   | 0.0438 | $4.51 \times 10^{-5}$ | 0.118              |
|          | 4096 | 24.5 ms          | 5.31 ms  | 0.0207             | 0.0158             | 0.0177 | 0.00809 | 0.0297 | $2.62 \times 10^{-7}$ | 0.0948             |
|          | 8192 | 24.7 ms          | 5.42 ms  | 0.0147             | 0.011              | 0.0124 | 0.00589 | 0.0212 | $2.5 \times 10^{-5}$  | 0.0638             |
| 10       | 2    | 24.8 ms          | 5.88 ms  | $1.95 \times 10^5$ | $6.17 \times 10^6$ | 8.99   | 8.94    | 9.08   | 8.93                  | $1.95 \times 10^8$ |
|          | 4    | 24.3 ms          | 5.69 ms  | 7.66               | 14.9               | 5.08   | 3.23    | 6.84   | 0.0203                | 245                |
|          | 8    | 24 ms            | 5.49 ms  | 4.65               | 6.22               | 3.47   | 1.88    | 5.13   | $1.99 \times 10^{-4}$ | 96.6               |
|          | 16   | 24.4 ms          | 5.75 ms  | 3                  | 2.99               | 2.42   | 1.26    | 3.79   | 0.00333               | 42.2               |
|          | 32   | 24.2 ms          | 5.69 ms  | 1.97               | 1.6                | 1.65   | 0.807   | 2.73   | 0.00466               | 15                 |
|          | 64   | 24.1 ms          | 5.55 ms  | 1.38               | 1.13               | 1.14   | 0.512   | 1.99   | 0.00131               | 8.3                |
|          | 128  | 24.1 ms          | 5.7 ms   | 0.953              | 0.745              | 0.786  | 0.367   | 1.38   | 0.00259               | 4.65               |
|          | 256  | 24.1 ms          | 5.73 ms  | 0.668              | 0.518              | 0.573  | 0.27    | 0.962  | $6.09 \times 10^{-4}$ | 3.63               |
|          | 512  | 24.2 ms          | 5.61 ms  | 0.481              | 0.353              | 0.427  | 0.194   | 0.692  | $1.53 \times 10^{-4}$ | 1.89               |
|          | 1024 | 24.1 ms          | 5.62 ms  | 0.331              | 0.249              | 0.282  | 0.134   | 0.471  | $1.48 \times 10^{-6}$ | 1.34               |
|          | 2048 | 24.1 ms          | 5.54 ms  | 0.233              | 0.173              | 0.197  | 0.0973  | 0.334  | 0.00107               | 1.08               |
|          | 4096 | 24.5 ms          | 5.8 ms   | 0.163              | 0.122              | 0.138  | 0.0687  | 0.233  | $5.06 \times 10^{-5}$ | 0.709              |
|          | 8192 | 24.4 ms          | 5.59 ms  | 0.117              | 0.0878             | 0.0971 | 0.0492  | 0.172  | $2.19 \times 10^{-5}$ | 0.527              |
| 100      | 2    | 28.5 ms          | 6.7 ms   | $5.18 \times 10^4$ | $1.28 \times 10^6$ | 98.9   | 98.9    | 98.9   | 98.9                  | $3.84 \times 10^7$ |
|          | 4    | 28.4 ms          | 6.66 ms  | 82                 | 204                | 65.8   | 42.7    | 79.4   | $5.83 \times 10^{-4}$ | 5030               |
|          | 8    | 27.4 ms          | 6.33 ms  | 47.9               | 57.6               | 38.2   | 20.7    | 56.1   | 0.0879                | 942                |
|          | 16   | 27.6 ms          | 6.37 ms  | 30.6               | 27.6               | 25.1   | 13      | 41.2   | 0.0041                | 339                |
|          | 32   | 27.7 ms          | 6.36 ms  | 21.4               | 18                 | 17.4   | 8.69    | 28.5   | 0.0269                | 129                |
|          | 64   | 27.3 ms          | 6.26 ms  | 14.7               | 11.6               | 12.5   | 5.92    | 20.9   | $6.86 \times 10^{-4}$ | 91.7               |
|          | 128  | 27.5 ms          | 6.46 ms  | 10.1               | 8.11               | 8.26   | 3.86    | 14.3   | 0.0121                | 51.9               |
|          | 256  | 27.4 ms          | 6.36 ms  | 7.2                | 5.61               | 6.14   | 2.85    | 10.3   | 0.00282               | 47                 |
|          | 512  | 27.4 ms          | 6.22 ms  | 4.96               | 3.88               | 4.31   | 1.77    | 7.3    | 0.0128                | 27                 |
|          | 1024 | 27.3 ms          | 6.42 ms  | 3.43               | 2.59               | 2.91   | 1.37    | 4.83   | 0.0197                | 14.2               |
|          | 2048 | 27.6 ms          | 6.3 ms   | 2.55               | 1.86               | 2.17   | 1.07    | 3.66   | $7.37 \times 10^{-4}$ | 10.6               |
|          | 4096 | 27.8 ms          | 6.19 ms  | 1.83               | 1.41               | 1.47   | 0.742   | 2.65   | 0.00109               | 8.48               |
|          | 8192 | 27.9 ms          | 6.35 ms  | 1.28               | 1.01               | 1.05   | 0.494   | 1.82   | 0.00355               | 5.87               |

Table 9: **Simulation study.** Results for estimator MML-3. Mean, standard deviation, median, [0.25, 0.75] quantile, min and max of absolute error.

| $\kappa$ | $N$  | Computation time |           | mean   | std. dev. | median | Error   |        | min                   | max    |
|----------|------|------------------|-----------|--------|-----------|--------|---------|--------|-----------------------|--------|
|          |      | mean             | std. dev. |        |           |        | 0.25    | 0.75   |                       |        |
| 0        | 2    | 23.7 ms          | 5.43 ms   | 0.582  | 0.375     | 0.559  | 0.238   | 0.922  | $6.69 \times 10^{-6}$ | 1.18   |
|          | 4    | 23.6 ms          | 5.35 ms   | 0.609  | 0.525     | 0.478  | 0.289   | 0.746  | 0.00749               | 5.81   |
|          | 8    | 23.6 ms          | 5.29 ms   | 0.497  | 0.316     | 0.434  | 0.278   | 0.623  | 0.018                 | 2.36   |
|          | 16   | 23.5 ms          | 5.19 ms   | 0.372  | 0.216     | 0.339  | 0.215   | 0.485  | 0.0132                | 1.33   |
|          | 32   | 23.5 ms          | 5.22 ms   | 0.275  | 0.152     | 0.251  | 0.161   | 0.361  | 0.00412               | 0.865  |
|          | 64   | 23.3 ms          | 5.11 ms   | 0.212  | 0.107     | 0.197  | 0.134   | 0.275  | 0.00479               | 0.739  |
|          | 128  | 23.6 ms          | 5.46 ms   | 0.153  | 0.0779    | 0.145  | 0.0941  | 0.199  | 0.00451               | 0.442  |
|          | 256  | 23.5 ms          | 5.3 ms    | 0.106  | 0.0569    | 0.0973 | 0.0639  | 0.14   | 0.00462               | 0.319  |
|          | 512  | 23.3 ms          | 5.19 ms   | 0.0751 | 0.0393    | 0.0713 | 0.0451  | 0.101  | 0.00281               | 0.205  |
|          | 1024 | 23.6 ms          | 5.4 ms    | 0.055  | 0.0286    | 0.0515 | 0.0338  | 0.0728 | 0.00108               | 0.164  |
|          | 2048 | 23.4 ms          | 5.17 ms   | 0.0399 | 0.0203    | 0.0384 | 0.0243  | 0.0522 | 0.0019                | 0.115  |
|          | 4096 | 23.7 ms          | 5.39 ms   | 0.028  | 0.0143    | 0.0262 | 0.017   | 0.0372 | $2.2 \times 10^{-4}$  | 0.0861 |
|          | 8192 | 23.6 ms          | 5.22 ms   | 0.0198 | 0.00995   | 0.0188 | 0.0121  | 0.0259 | $2.87 \times 10^{-4}$ | 0.0604 |
| 0.01     | 2    | 24 ms            | 5.64 ms   | 0.586  | 0.374     | 0.559  | 0.243   | 0.917  | $2.42 \times 10^{-4}$ | 1.17   |
|          | 4    | 23.9 ms          | 5.88 ms   | 0.616  | 0.518     | 0.477  | 0.285   | 0.76   | 0.0018                | 3.84   |
|          | 8    | 24 ms            | 5.65 ms   | 0.483  | 0.312     | 0.418  | 0.257   | 0.652  | 0.0083                | 2.06   |
|          | 16   | 23.6 ms          | 5.4 ms    | 0.373  | 0.218     | 0.342  | 0.216   | 0.487  | $7.15 \times 10^{-4}$ | 1.49   |
|          | 32   | 23.8 ms          | 5.48 ms   | 0.278  | 0.155     | 0.258  | 0.161   | 0.374  | 0.00128               | 1.11   |
|          | 64   | 23.5 ms          | 5.36 ms   | 0.205  | 0.108     | 0.192  | 0.121   | 0.27   | 0.00532               | 0.583  |
|          | 128  | 23.4 ms          | 5.25 ms   | 0.148  | 0.0855    | 0.138  | 0.0835  | 0.198  | $2.67 \times 10^{-4}$ | 0.505  |
|          | 256  | 23.5 ms          | 5.52 ms   | 0.102  | 0.0575    | 0.0928 | 0.0607  | 0.137  | $6.79 \times 10^{-5}$ | 0.302  |
|          | 512  | 23.3 ms          | 5.26 ms   | 0.0683 | 0.04      | 0.0629 | 0.0388  | 0.0931 | $5.83 \times 10^{-4}$ | 0.205  |
|          | 1024 | 23.8 ms          | 5.58 ms   | 0.0463 | 0.0292    | 0.0431 | 0.0237  | 0.0641 | $3.28 \times 10^{-5}$ | 0.148  |
|          | 2048 | 23.8 ms          | 5.45 ms   | 0.0301 | 0.0205    | 0.0275 | 0.0137  | 0.0424 | $3.62 \times 10^{-5}$ | 0.113  |
|          | 4096 | 23.7 ms          | 5.23 ms   | 0.0193 | 0.0139    | 0.0173 | 0.00745 | 0.0284 | $3.25 \times 10^{-5}$ | 0.0651 |
|          | 8192 | 23.7 ms          | 5.36 ms   | 0.0128 | 0.00962   | 0.0107 | 0.00487 | 0.019  | $2.9 \times 10^{-5}$  | 0.0517 |
| 0.1      | 2    | 24.1 ms          | 5.59 ms   | 0.525  | 0.354     | 0.516  | 0.19    | 0.855  | $4.3 \times 10^{-4}$  | 1.08   |
|          | 4    | 23.8 ms          | 5.65 ms   | 0.539  | 0.496     | 0.411  | 0.221   | 0.671  | $1.55 \times 10^{-4}$ | 4.48   |
|          | 8    | 23.7 ms          | 5.53 ms   | 0.397  | 0.319     | 0.317  | 0.172   | 0.536  | $3.73 \times 10^{-4}$ | 1.84   |
|          | 16   | 23.6 ms          | 5.4 ms    | 0.307  | 0.231     | 0.267  | 0.127   | 0.421  | $3.79 \times 10^{-4}$ | 1.4    |
|          | 32   | 23.4 ms          | 5.27 ms   | 0.211  | 0.158     | 0.186  | 0.0789  | 0.308  | $6.72 \times 10^{-4}$ | 1.02   |
|          | 64   | 23.7 ms          | 5.59 ms   | 0.136  | 0.11      | 0.113  | 0.047   | 0.197  | $5.25 \times 10^{-4}$ | 0.578  |
|          | 128  | 23.8 ms          | 5.8 ms    | 0.0893 | 0.0741    | 0.0694 | 0.0319  | 0.127  | $1.03 \times 10^{-4}$ | 0.406  |
|          | 256  | 23.5 ms          | 5.46 ms   | 0.0642 | 0.052     | 0.0524 | 0.0241  | 0.0907 | $2.17 \times 10^{-5}$ | 0.301  |
|          | 512  | 23.7 ms          | 5.23 ms   | 0.0472 | 0.0364    | 0.0405 | 0.018   | 0.0679 | $8.45 \times 10^{-5}$ | 0.22   |
|          | 1024 | 23.6 ms          | 5.4 ms    | 0.0341 | 0.0259    | 0.0286 | 0.0145  | 0.0482 | $7.77 \times 10^{-6}$ | 0.153  |
|          | 2048 | 23.7 ms          | 5.46 ms   | 0.0248 | 0.0191    | 0.021  | 0.00945 | 0.0359 | $1.75 \times 10^{-5}$ | 0.107  |
|          | 4096 | 23.8 ms          | 5.42 ms   | 0.0174 | 0.0132    | 0.0145 | 0.00707 | 0.0256 | $2.81 \times 10^{-6}$ | 0.0676 |
|          | 8192 | 24.2 ms          | 5.51 ms   | 0.0131 | 0.00949   | 0.0115 | 0.00564 | 0.0192 | $2.73 \times 10^{-5}$ | 0.0568 |
| 1        | 2    | 24.3 ms          | 5.47 ms   | 0.377  | 0.296     | 0.272  | 0.13    | 0.631  | $1.68 \times 10^{-4}$ | 1      |
|          | 4    | 24.3 ms          | 5.52 ms   | 0.582  | 0.632     | 0.478  | 0.246   | 0.706  | 0.00143               | 6.29   |
|          | 8    | 24.1 ms          | 5.45 ms   | 0.421  | 0.42      | 0.332  | 0.164   | 0.585  | 0.00147               | 5.68   |
|          | 16   | 24.2 ms          | 5.59 ms   | 0.326  | 0.255     | 0.28   | 0.132   | 0.463  | $2.84 \times 10^{-4}$ | 2      |
|          | 32   | 24.4 ms          | 5.59 ms   | 0.238  | 0.187     | 0.203  | 0.0924  | 0.332  | $2.52 \times 10^{-4}$ | 1.26   |
|          | 64   | 24.1 ms          | 5.36 ms   | 0.168  | 0.132     | 0.144  | 0.0613  | 0.237  | $2.8 \times 10^{-4}$  | 0.848  |
|          | 128  | 24.1 ms          | 5.43 ms   | 0.118  | 0.0902    | 0.101  | 0.0463  | 0.173  | $1.54 \times 10^{-4}$ | 0.59   |
|          | 256  | 24.1 ms          | 5.42 ms   | 0.0832 | 0.0644    | 0.0671 | 0.0312  | 0.121  | $5.12 \times 10^{-4}$ | 0.304  |
|          | 512  | 24.5 ms          | 5.66 ms   | 0.0593 | 0.0457    | 0.0484 | 0.0227  | 0.086  | $1.03 \times 10^{-5}$ | 0.246  |
|          | 1024 | 24.2 ms          | 5.39 ms   | 0.0416 | 0.0319    | 0.036  | 0.016   | 0.0599 | $1.84 \times 10^{-5}$ | 0.171  |
|          | 2048 | 24.2 ms          | 5.49 ms   | 0.0305 | 0.0226    | 0.0262 | 0.012   | 0.0438 | $9.67 \times 10^{-7}$ | 0.118  |
|          | 4096 | 24.5 ms          | 5.55 ms   | 0.0207 | 0.0158    | 0.0177 | 0.00809 | 0.0297 | $2.62 \times 10^{-7}$ | 0.0949 |
|          | 8192 | 24.7 ms          | 5.71 ms   | 0.0147 | 0.011     | 0.0124 | 0.00589 | 0.0212 | $5.83 \times 10^{-5}$ | 0.0638 |
| 10       | 2    | 23.9 ms          | 5.25 ms   | 8.9    | 0.103     | 8.86   | 8.83    | 8.94   | 8.82                  | 9.43   |
|          | 4    | 23.6 ms          | 5.33 ms   | 6.23   | 1.59      | 6.63   | 5.63    | 7.31   | 0.0069                | 9      |
|          | 8    | 23.8 ms          | 5.21 ms   | 4.54   | 4.55      | 4.11   | 2.4     | 5.58   | 0.00715               | 75.5   |
|          | 16   | 23.9 ms          | 5.52 ms   | 2.99   | 2.63      | 2.68   | 1.31    | 3.99   | 0.00487               | 38.2   |
|          | 32   | 24.1 ms          | 5.48 ms   | 1.97   | 1.51      | 1.76   | 0.86    | 2.78   | 0.00196               | 14.2   |
|          | 64   | 23.8 ms          | 5.3 ms    | 1.38   | 1.1       | 1.16   | 0.534   | 1.98   | $5.21 \times 10^{-4}$ | 8.01   |
|          | 128  | 23.5 ms          | 5.3 ms    | 0.949  | 0.735     | 0.788  | 0.37    | 1.39   | $8.88 \times 10^{-4}$ | 4.53   |
|          | 256  | 23.7 ms          | 5.3 ms    | 0.665  | 0.514     | 0.578  | 0.273   | 0.957  | 0.0021                | 3.58   |
|          | 512  | 23.9 ms          | 5.61 ms   | 0.48   | 0.351     | 0.423  | 0.195   | 0.682  | $6.44 \times 10^{-4}$ | 1.87   |
|          | 1024 | 23.9 ms          | 5.45 ms   | 0.33   | 0.249     | 0.28   | 0.129   | 0.474  | $7.4 \times 10^{-4}$  | 1.33   |
|          | 2048 | 23.6 ms          | 5.06 ms   | 0.233  | 0.173     | 0.196  | 0.097   | 0.334  | $6.45 \times 10^{-5}$ | 1.08   |
|          | 4096 | 23.8 ms          | 5.34 ms   | 0.163  | 0.122     | 0.138  | 0.0692  | 0.234  | $4.34 \times 10^{-4}$ | 0.711  |
|          | 8192 | 24 ms            | 5.31 ms   | 0.117  | 0.0878    | 0.0967 | 0.0487  | 0.172  | $2.66 \times 10^{-4}$ | 0.526  |
| 100      | 2    | 25.7 ms          | 5.73 ms   | 98.8   | 0.0132    | 98.8   | 98.8    | 98.8   | 98.8                  | 98.9   |
|          | 4    | 25.2 ms          | 5.74 ms   | 90.5   | 5.09      | 91.8   | 89.3    | 93.4   | 26                    | 96.5   |
|          | 8    | 25.1 ms          | 5.68 ms   | 47.1   | 42.3      | 44.9   | 26      | 59.8   | 0.23                  | 734    |
|          | 16   | 25.2 ms          | 5.71 ms   | 30     | 24.1      | 26.3   | 14.3    | 40     | 0.00708               | 306    |
|          | 32   | 25.3 ms          | 5.95 ms   | 21     | 16.9      | 17.7   | 8.49    | 29.5   | 0.0466                | 121    |
|          | 64   | 24.9 ms          | 5.58 ms   | 14.6   | 11.3      | 12.6   | 6       | 20.9   | 0.0299                | 88.5   |
|          | 128  | 24.8 ms          | 5.43 ms   | 10     | 7.96      | 8.37   | 3.89    | 14.5   | 0.0254                | 50.7   |
|          | 256  | 24.9 ms          | 5.46 ms   | 7.2    | 5.55      | 6.11   | 2.95    | 10.3   | 0.00885               | 46.4   |
|          | 512  | 25.1 ms          | 5.69 ms   | 4.95   | 3.86      | 4.27   | 1.78    | 7.18   | $8.98 \times 10^{-4}$ | 26.8   |
|          | 1024 | 25.3 ms          | 5.76 ms   | 3.43   | 2.58      | 2.92   | 1.39    | 4.85   | 0.00656               | 14.1   |
|          | 2048 | 25.5 ms          | 5.81 ms   | 2.56   | 1.86      | 2.16   | 1.07    | 3.65   | 0.00967               | 10.5   |
|          | 4096 | 25.2 ms          | 5.63 ms   | 1.83   | 1.41      | 1.48   | 0.732   | 2.65   | 0.00555               | 8.45   |
|          | 8192 | 25.3 ms          | 5.77 ms   | 1.28   | 1.01      | 1.05   | 0.484   | 1.82   | 0.00436               | 5.86   |

Table 10: **Simulation study.** Results for estimator **BayesEst-2-km**. Mean, standard deviation, median,  $[0.25, 0.75]$  quantile, min and max of absolute error.

| $\kappa$ | $N$  | Computation time |           | mean   | std. dev. | median | Error   |        |                       |        |
|----------|------|------------------|-----------|--------|-----------|--------|---------|--------|-----------------------|--------|
|          |      | mean             | std. dev. |        |           |        | 0.25    | 0.75   | min                   | max    |
| 0        | 2    | 22.7 ms          | 4.18 ms   | 1.06   | 0.367     | 0.998  | 0.713   | 1.38   | 0.554                 | 1.68   |
|          | 4    | 22.9 ms          | 4.5 ms    | 0.935  | 0.479     | 0.803  | 0.657   | 1.03   | 0.481                 | 6.19   |
|          | 8    | 22.7 ms          | 4.32 ms   | 0.732  | 0.259     | 0.669  | 0.556   | 0.819  | 0.4                   | 2.44   |
|          | 16   | 22.6 ms          | 4 ms      | 0.551  | 0.168     | 0.516  | 0.43    | 0.629  | 0.313                 | 1.39   |
|          | 32   | 22.8 ms          | 4.4 ms    | 0.41   | 0.116     | 0.385  | 0.323   | 0.469  | 0.233                 | 0.913  |
|          | 64   | 22.8 ms          | 4.38 ms   | 0.308  | 0.0821    | 0.293  | 0.248   | 0.353  | 0.172                 | 0.77   |
|          | 128  | 22.6 ms          | 4.01 ms   | 0.223  | 0.0601    | 0.214  | 0.178   | 0.256  | 0.125                 | 0.471  |
|          | 256  | 22.4 ms          | 3.92 ms   | 0.157  | 0.0439    | 0.148  | 0.125   | 0.181  | 0.0898                | 0.34   |
|          | 512  | 22.6 ms          | 4.21 ms   | 0.112  | 0.0302    | 0.107  | 0.0886  | 0.13   | 0.0636                | 0.222  |
|          | 1024 | 22.8 ms          | 4.32 ms   | 0.0808 | 0.0222    | 0.0767 | 0.0641  | 0.0935 | 0.0446                | 0.175  |
|          | 2048 | 22.4 ms          | 3.81 ms   | 0.0579 | 0.0158    | 0.0558 | 0.0456  | 0.0667 | 0.0322                | 0.123  |
|          | 4096 | 22.6 ms          | 4.03 ms   | 0.0408 | 0.0112    | 0.0388 | 0.0322  | 0.0475 | 0.0222                | 0.0914 |
|          | 8192 | 23 ms            | 4.08 ms   | 0.0288 | 0.00774   | 0.0276 | 0.0228  | 0.0332 | 0.0158                | 0.0642 |
| 0.01     | 2    | 24 ms            | 5.35 ms   | 1.06   | 0.368     | 0.999  | 0.715   | 1.38   | 0.544                 | 1.67   |
|          | 4    | 23.6 ms          | 5.3 ms    | 0.94   | 0.466     | 0.8    | 0.652   | 1.04   | 0.474                 | 4.1    |
|          | 8    | 24 ms            | 5.51 ms   | 0.719  | 0.253     | 0.654  | 0.538   | 0.841  | 0.391                 | 2.15   |
|          | 16   | 23.8 ms          | 5.21 ms   | 0.549  | 0.171     | 0.516  | 0.427   | 0.628  | 0.3                   | 1.54   |
|          | 32   | 24.2 ms          | 5.81 ms   | 0.41   | 0.12      | 0.387  | 0.319   | 0.478  | 0.225                 | 1.14   |
|          | 64   | 24 ms            | 5.55 ms   | 0.301  | 0.0833    | 0.286  | 0.236   | 0.347  | 0.161                 | 0.622  |
|          | 128  | 24.1 ms          | 5.7 ms    | 0.218  | 0.0669    | 0.206  | 0.167   | 0.253  | 0.115                 | 0.529  |
|          | 256  | 24.2 ms          | 5.93 ms   | 0.152  | 0.0449    | 0.142  | 0.119   | 0.177  | 0.0794                | 0.323  |
|          | 512  | 24.1 ms          | 5.6 ms    | 0.104  | 0.0311    | 0.0984 | 0.0811  | 0.122  | 0.0527                | 0.221  |
|          | 1024 | 23.9 ms          | 5.3 ms    | 0.0717 | 0.0229    | 0.068  | 0.054   | 0.0845 | 0.035                 | 0.159  |
|          | 2048 | 23.9 ms          | 5.41 ms   | 0.0479 | 0.0164    | 0.0452 | 0.0352  | 0.0569 | 0.0224                | 0.12   |
|          | 4096 | 23.9 ms          | 5.34 ms   | 0.0313 | 0.0116    | 0.0296 | 0.0222  | 0.0385 | 0.0125                | 0.0711 |
|          | 8192 | 24.7 ms          | 5.8 ms    | 0.0204 | 0.00857   | 0.0191 | 0.0139  | 0.0258 | 0.00616               | 0.0555 |
| 0.1      | 2    | 24.2 ms          | 5.66 ms   | 0.989  | 0.36      | 0.955  | 0.655   | 1.32   | 0.455                 | 1.58   |
|          | 4    | 23.9 ms          | 5.51 ms   | 0.857  | 0.449     | 0.73   | 0.581   | 0.952  | 0.386                 | 4.79   |
|          | 8    | 24.2 ms          | 5.8 ms    | 0.631  | 0.263     | 0.556  | 0.452   | 0.729  | 0.295                 | 1.93   |
|          | 16   | 23.8 ms          | 5.43 ms   | 0.476  | 0.188     | 0.437  | 0.338   | 0.558  | 0.214                 | 1.45   |
|          | 32   | 24.2 ms          | 5.63 ms   | 0.334  | 0.129     | 0.311  | 0.234   | 0.407  | 0.133                 | 1.05   |
|          | 64   | 23.7 ms          | 5.21 ms   | 0.221  | 0.0946    | 0.204  | 0.151   | 0.271  | 0.0791                | 0.612  |
|          | 128  | 23.9 ms          | 5.49 ms   | 0.14   | 0.0706    | 0.128  | 0.0878  | 0.179  | 0.0238                | 0.431  |
|          | 256  | 23.7 ms          | 5.52 ms   | 0.0881 | 0.0566    | 0.0796 | 0.0448  | 0.124  | $4.36 \times 10^{-6}$ | 0.318  |
|          | 512  | 24.1 ms          | 5.81 ms   | 0.0552 | 0.0411    | 0.0466 | 0.0223  | 0.0808 | $6.08 \times 10^{-5}$ | 0.231  |
|          | 1024 | 23.8 ms          | 5.28 ms   | 0.0361 | 0.0279    | 0.0317 | 0.0148  | 0.0497 | $1.75 \times 10^{-4}$ | 0.161  |
|          | 2048 | 23.8 ms          | 5.25 ms   | 0.0254 | 0.0196    | 0.0206 | 0.0102  | 0.0364 | $8.02 \times 10^{-5}$ | 0.111  |
|          | 4096 | 24.1 ms          | 5.57 ms   | 0.0177 | 0.0133    | 0.0155 | 0.007   | 0.0255 | $4.36 \times 10^{-5}$ | 0.0704 |
|          | 8192 | 24 ms            | 5.42 ms   | 0.0133 | 0.00952   | 0.0118 | 0.00551 | 0.0193 | $5.97 \times 10^{-5}$ | 0.0517 |
| 1        | 2    | 24.6 ms          | 5.91 ms   | 0.348  | 0.204     | 0.335  | 0.177   | 0.524  | $3.57 \times 10^{-4}$ | 0.684  |
|          | 4    | 24.1 ms          | 5.44 ms   | 0.5    | 0.719     | 0.281  | 0.152   | 0.495  | 0.00114               | 6.72   |
|          | 8    | 24.1 ms          | 5.53 ms   | 0.361  | 0.429     | 0.256  | 0.122   | 0.44   | $8.8 \times 10^{-4}$  | 5.73   |
|          | 16   | 24 ms            | 5.29 ms   | 0.292  | 0.252     | 0.237  | 0.107   | 0.397  | $1.48 \times 10^{-4}$ | 2.04   |
|          | 32   | 24.3 ms          | 5.55 ms   | 0.223  | 0.184     | 0.181  | 0.0845  | 0.316  | $6.29 \times 10^{-4}$ | 1.28   |
|          | 64   | 24.2 ms          | 5.47 ms   | 0.162  | 0.13      | 0.136  | 0.0612  | 0.226  | $7.56 \times 10^{-5}$ | 0.858  |
|          | 128  | 23.8 ms          | 5.32 ms   | 0.117  | 0.0893    | 0.1    | 0.0448  | 0.168  | $1.14 \times 10^{-4}$ | 0.596  |
|          | 256  | 23.6 ms          | 5.01 ms   | 0.0825 | 0.0641    | 0.067  | 0.032   | 0.119  | $5.1 \times 10^{-4}$  | 0.308  |
|          | 512  | 24.1 ms          | 5.59 ms   | 0.0589 | 0.0457    | 0.0494 | 0.0233  | 0.0857 | $3.03 \times 10^{-5}$ | 0.248  |
|          | 1024 | 23.9 ms          | 5.38 ms   | 0.0415 | 0.0319    | 0.0357 | 0.017   | 0.0595 | $8.17 \times 10^{-5}$ | 0.172  |
|          | 2048 | 24.1 ms          | 5.45 ms   | 0.0305 | 0.0226    | 0.0259 | 0.012   | 0.0437 | $3.62 \times 10^{-5}$ | 0.119  |
|          | 4096 | 24 ms            | 5.19 ms   | 0.0207 | 0.0158    | 0.0178 | 0.00818 | 0.0296 | $5.6 \times 10^{-5}$  | 0.0951 |
|          | 8192 | 24.1 ms          | 5.36 ms   | 0.0147 | 0.011     | 0.0125 | 0.00597 | 0.0212 | $1.87 \times 10^{-5}$ | 0.064  |
| 10       | 2    | 24.2 ms          | 5.3 ms    | 8.41   | 0.118     | 8.37   | 8.33    | 8.46   | 8.32                  | 8.99   |
|          | 4    | 24 ms            | 5.51 ms   | 5.99   | 1.6       | 6.38   | 5.33    | 7.09   | 0.092                 | 8.74   |
|          | 8    | 24.3 ms          | 5.77 ms   | 4.5    | 4.55      | 4.05   | 2.38    | 5.51   | 0.003                 | 75.5   |
|          | 16   | 24 ms            | 5.64 ms   | 2.98   | 2.63      | 2.66   | 1.31    | 3.98   | 0.00344               | 38.2   |
|          | 32   | 23.9 ms          | 5.31 ms   | 1.97   | 1.51      | 1.75   | 0.855   | 2.78   | $2.28 \times 10^{-4}$ | 14.2   |
|          | 64   | 23.6 ms          | 5.35 ms   | 1.38   | 1.1       | 1.15   | 0.531   | 1.98   | 0.00117               | 8.01   |
|          | 128  | 24 ms            | 5.51 ms   | 0.948  | 0.734     | 0.787  | 0.369   | 1.39   | $1.88 \times 10^{-4}$ | 4.53   |
|          | 256  | 23.5 ms          | 5.1 ms    | 0.665  | 0.514     | 0.578  | 0.272   | 0.957  | 0.00137               | 3.58   |
|          | 512  | 23.9 ms          | 5.42 ms   | 0.48   | 0.351     | 0.423  | 0.195   | 0.682  | 0.00101               | 1.87   |
|          | 1024 | 24.1 ms          | 5.5 ms    | 0.33   | 0.249     | 0.28   | 0.129   | 0.473  | $4.97 \times 10^{-4}$ | 1.33   |
|          | 2048 | 24.3 ms          | 5.64 ms   | 0.233  | 0.173     | 0.196  | 0.0969  | 0.334  | $3.81 \times 10^{-6}$ | 1.08   |
|          | 4096 | 24.2 ms          | 5.62 ms   | 0.163  | 0.122     | 0.138  | 0.0692  | 0.234  | $4.94 \times 10^{-4}$ | 0.711  |
|          | 8192 | 24.5 ms          | 5.58 ms   | 0.117  | 0.0878    | 0.0967 | 0.0488  | 0.172  | $2.66 \times 10^{-4}$ | 0.526  |
| 100      | 2    | 25.9 ms          | 6.12 ms   | 98.3   | 0.0158    | 98.3   | 98.3    | 98.3   | 98.3                  | 98.4   |
|          | 4    | 25.4 ms          | 5.8 ms    | 90     | 5.18      | 91.3   | 88.8    | 93     | 25.1                  | 96.2   |
|          | 8    | 25.3 ms          | 5.91 ms   | 47.1   | 42.3      | 44.9   | 26      | 59.8   | 0.225                 | 734    |
|          | 16   | 25.1 ms          | 5.73 ms   | 30     | 24.1      | 26.3   | 14.3    | 40     | 0.00542               | 306    |
|          | 32   | 24.9 ms          | 5.87 ms   | 21     | 16.9      | 17.7   | 8.49    | 29.5   | 0.0458                | 121    |
|          | 64   | 24.9 ms          | 5.68 ms   | 14.6   | 11.3      | 12.6   | 6       | 20.9   | 0.0296                | 88.5   |
|          | 128  | 25 ms            | 5.61 ms   | 10     | 7.96      | 8.37   | 3.89    | 14.5   | 0.0252                | 50.7   |
|          | 256  | 24.8 ms          | 5.67 ms   | 7.2    | 5.55      | 6.11   | 2.95    | 10.3   | 0.00877               | 46.4   |
|          | 512  | 25 ms            | 5.76 ms   | 4.95   | 3.86      | 4.27   | 1.78    | 7.18   | $8.98 \times 10^{-4}$ | 26.8   |
|          | 1024 | 25.2 ms          | 5.84 ms   | 3.43   | 2.58      | 2.92   | 1.39    | 4.85   | 0.00656               | 14.1   |
|          | 2048 | 24.9 ms          | 5.59 ms   | 2.56   | 1.86      | 2.16   | 1.07    | 3.65   | 0.0096                | 10.5   |
|          | 4096 | 25 ms            | 5.63 ms   | 1.83   | 1.41      | 1.48   | 0.732   | 2.65   | 0.00555               | 8.45   |
|          | 8192 | 25.7 ms          | 5.97 ms   | 1.28   | 1.01      | 1.05   | 0.484   | 1.82   | 0.00436               | 5.86   |

Table 11: **Simulation study.** Results for estimator BayesEst-3-km. Mean, standard deviation, median, [0.25, 0.75] quantile, min and max of absolute error.

| $\kappa$ | $N$  | Computation time |           | mean   | std. dev. | median | Error   |        |                       |        |
|----------|------|------------------|-----------|--------|-----------|--------|---------|--------|-----------------------|--------|
|          |      | mean             | std. dev. |        |           |        | 0.25    | 0.75   | min                   | max    |
| 0        | 2    | 22.6 ms          | 4.22 ms   | 0.368  | 0.21      | 0.387  | 0.176   | 0.567  | $6.69 \times 10^{-6}$ | 0.657  |
|          | 4    | 22.5 ms          | 3.94 ms   | 0.439  | 0.303     | 0.371  | 0.228   | 0.559  | 0.00599               | 1.94   |
|          | 8    | 22.4 ms          | 3.73 ms   | 0.42   | 0.263     | 0.369  | 0.238   | 0.527  | 0.0155                | 1.93   |
|          | 16   | 22.5 ms          | 3.99 ms   | 0.339  | 0.197     | 0.309  | 0.196   | 0.442  | 0.012                 | 1.22   |
|          | 32   | 22.6 ms          | 4.18 ms   | 0.261  | 0.145     | 0.238  | 0.153   | 0.342  | 0.00389               | 0.826  |
|          | 64   | 22.3 ms          | 3.91 ms   | 0.206  | 0.104     | 0.192  | 0.13    | 0.268  | 0.00466               | 0.721  |
|          | 128  | 22.4 ms          | 4.02 ms   | 0.151  | 0.0768    | 0.143  | 0.0927  | 0.196  | 0.00445               | 0.436  |
|          | 256  | 22.3 ms          | 3.94 ms   | 0.105  | 0.0565    | 0.0966 | 0.0634  | 0.139  | 0.00462               | 0.316  |
|          | 512  | 22.4 ms          | 4.27 ms   | 0.0748 | 0.0392    | 0.071  | 0.0449  | 0.1    | 0.00281               | 0.204  |
|          | 1024 | 22.5 ms          | 4.21 ms   | 0.0549 | 0.0286    | 0.0514 | 0.0338  | 0.0727 | 0.00108               | 0.164  |
|          | 2048 | 22.4 ms          | 4.07 ms   | 0.0399 | 0.0203    | 0.0384 | 0.0242  | 0.0522 | 0.0019                | 0.115  |
|          | 4096 | 22.3 ms          | 3.71 ms   | 0.028  | 0.0143    | 0.0262 | 0.017   | 0.0372 | $2.2 \times 10^{-4}$  | 0.0861 |
|          | 8192 | 22.5 ms          | 4 ms      | 0.0198 | 0.00995   | 0.0188 | 0.0121  | 0.0259 | $2.87 \times 10^{-4}$ | 0.0604 |
| 0.01     | 2    | 24.2 ms          | 5.47 ms   | 0.366  | 0.208     | 0.383  | 0.177   | 0.559  | $7.2 \times 10^{-4}$  | 0.647  |
|          | 4    | 24 ms            | 5.51 ms   | 0.441  | 0.314     | 0.368  | 0.223   | 0.565  | $5.71 \times 10^{-4}$ | 1.78   |
|          | 8    | 24.3 ms          | 5.58 ms   | 0.407  | 0.26      | 0.354  | 0.218   | 0.549  | 0.00571               | 1.7    |
|          | 16   | 23.8 ms          | 5.36 ms   | 0.338  | 0.199     | 0.31   | 0.196   | 0.442  | 0.00152               | 1.37   |
|          | 32   | 24 ms            | 5.64 ms   | 0.263  | 0.148     | 0.244  | 0.152   | 0.355  | 0.00171               | 1.06   |
|          | 64   | 24 ms            | 5.55 ms   | 0.199  | 0.105     | 0.186  | 0.118   | 0.262  | 0.00486               | 0.568  |
|          | 128  | 23.6 ms          | 5.35 ms   | 0.146  | 0.0843    | 0.136  | 0.0822  | 0.195  | $1.33 \times 10^{-4}$ | 0.498  |
|          | 256  | 23.2 ms          | 5.03 ms   | 0.101  | 0.0571    | 0.0921 | 0.0601  | 0.136  | $1.31 \times 10^{-4}$ | 0.299  |
|          | 512  | 23.8 ms          | 5.52 ms   | 0.068  | 0.0399    | 0.0627 | 0.0386  | 0.0927 | $6.43 \times 10^{-4}$ | 0.204  |
|          | 1024 | 23.6 ms          | 5.37 ms   | 0.0462 | 0.0291    | 0.0431 | 0.0237  | 0.0639 | $3.03 \times 10^{-5}$ | 0.148  |
|          | 2048 | 23.7 ms          | 5.5 ms    | 0.0301 | 0.0205    | 0.0275 | 0.0136  | 0.0424 | $3.62 \times 10^{-5}$ | 0.113  |
|          | 4096 | 24.1 ms          | 5.58 ms   | 0.0193 | 0.0139    | 0.0173 | 0.00745 | 0.0284 | $3.25 \times 10^{-5}$ | 0.0651 |
|          | 8192 | 24.1 ms          | 5.61 ms   | 0.0128 | 0.00962   | 0.0107 | 0.00487 | 0.019  | $2.9 \times 10^{-5}$  | 0.0517 |
| 0.1      | 2    | 24.7 ms          | 5.71 ms   | 0.299  | 0.187     | 0.32   | 0.113   | 0.48   | $1.3 \times 10^{-4}$  | 0.557  |
|          | 4    | 24.4 ms          | 5.53 ms   | 0.364  | 0.298     | 0.295  | 0.153   | 0.476  | $1.23 \times 10^{-5}$ | 1.77   |
|          | 8    | 24.4 ms          | 5.53 ms   | 0.322  | 0.265     | 0.255  | 0.132   | 0.438  | $5.96 \times 10^{-5}$ | 1.51   |
|          | 16   | 24.3 ms          | 5.34 ms   | 0.272  | 0.211     | 0.234  | 0.107   | 0.374  | $3.1 \times 10^{-4}$  | 1.28   |
|          | 32   | 24 ms            | 5.17 ms   | 0.196  | 0.15      | 0.171  | 0.0696  | 0.288  | $1.57 \times 10^{-4}$ | 0.97   |
|          | 64   | 24.1 ms          | 5.51 ms   | 0.131  | 0.106     | 0.107  | 0.0452  | 0.189  | $2.41 \times 10^{-5}$ | 0.562  |
|          | 128  | 24.2 ms          | 5.54 ms   | 0.0872 | 0.0726    | 0.0681 | 0.032   | 0.124  | $6.24 \times 10^{-5}$ | 0.399  |
|          | 256  | 24.3 ms          | 5.4 ms    | 0.0634 | 0.0514    | 0.052  | 0.0233  | 0.0896 | $2.8 \times 10^{-4}$  | 0.298  |
|          | 512  | 24 ms            | 5.26 ms   | 0.0469 | 0.0362    | 0.0401 | 0.0177  | 0.0676 | $8.39 \times 10^{-5}$ | 0.219  |
|          | 1024 | 24.2 ms          | 5.39 ms   | 0.0339 | 0.0259    | 0.0285 | 0.0146  | 0.048  | $9.02 \times 10^{-6}$ | 0.153  |
|          | 2048 | 24.1 ms          | 5.2 ms    | 0.0247 | 0.019     | 0.021  | 0.00947 | 0.0358 | $5.81 \times 10^{-6}$ | 0.107  |
|          | 4096 | 24.5 ms          | 5.46 ms   | 0.0174 | 0.0132    | 0.0145 | 0.00707 | 0.0256 | $2.81 \times 10^{-6}$ | 0.0675 |
|          | 8192 | 24.4 ms          | 5.21 ms   | 0.0131 | 0.0095    | 0.0115 | 0.00564 | 0.0192 | $2.73 \times 10^{-5}$ | 0.0568 |
| 1        | 2    | 24.5 ms          | 5.48 ms   | 0.571  | 0.199     | 0.521  | 0.386   | 0.733  | 0.343                 | 1      |
|          | 4    | 24.4 ms          | 5.56 ms   | 0.468  | 0.25      | 0.483  | 0.263   | 0.661  | $3.28 \times 10^{-4}$ | 0.976  |
|          | 8    | 24.3 ms          | 5.31 ms   | 0.401  | 0.304     | 0.364  | 0.179   | 0.562  | $8.63 \times 10^{-6}$ | 3.4    |
|          | 16   | 24.1 ms          | 5.15 ms   | 0.32   | 0.231     | 0.278  | 0.143   | 0.458  | $5.38 \times 10^{-4}$ | 1.72   |
|          | 32   | 24.2 ms          | 5.37 ms   | 0.237  | 0.178     | 0.209  | 0.0976  | 0.336  | $3.76 \times 10^{-4}$ | 1.17   |
|          | 64   | 24.1 ms          | 5.15 ms   | 0.168  | 0.129     | 0.141  | 0.0633  | 0.242  | $1.3 \times 10^{-4}$  | 0.812  |
|          | 128  | 24.1 ms          | 5.12 ms   | 0.118  | 0.0895    | 0.0983 | 0.0502  | 0.17   | $3.88 \times 10^{-4}$ | 0.575  |
|          | 256  | 23.9 ms          | 5.05 ms   | 0.0831 | 0.0643    | 0.0684 | 0.032   | 0.121  | $1.24 \times 10^{-4}$ | 0.297  |
|          | 512  | 24.2 ms          | 5.37 ms   | 0.0594 | 0.0456    | 0.048  | 0.0234  | 0.0865 | $4.74 \times 10^{-4}$ | 0.243  |
|          | 1024 | 24.3 ms          | 5.35 ms   | 0.0415 | 0.0319    | 0.0361 | 0.0157  | 0.0594 | $8.69 \times 10^{-5}$ | 0.17   |
|          | 2048 | 24.4 ms          | 5.35 ms   | 0.0304 | 0.0226    | 0.0262 | 0.012   | 0.044  | $1.49 \times 10^{-4}$ | 0.118  |
|          | 4096 | 24.5 ms          | 5.47 ms   | 0.0207 | 0.0158    | 0.0176 | 0.00799 | 0.0298 | $6.58 \times 10^{-5}$ | 0.0945 |
|          | 8192 | 24.6 ms          | 5.46 ms   | 0.0146 | 0.011     | 0.0124 | 0.00583 | 0.0211 | $1.72 \times 10^{-5}$ | 0.0636 |
| 10       | 2    | 24.1 ms          | 5.25 ms   | 9.37   | 0.0382    | 9.36   | 9.35    | 9.38   | 9.34                  | 9.61   |
|          | 4    | 24 ms            | 5.63 ms   | 8.33   | 0.223     | 8.29   | 8.15    | 8.47   | 7.98                  | 9.27   |
|          | 8    | 24.1 ms          | 5.56 ms   | 5.34   | 2.04      | 5.68   | 4.36    | 6.5    | 0.0352                | 33.5   |
|          | 16   | 24.2 ms          | 5.58 ms   | 3.24   | 2.09      | 3.24   | 1.83    | 4.41   | $5.51 \times 10^{-4}$ | 30.3   |
|          | 32   | 24 ms            | 5.5 ms    | 2.07   | 1.38      | 1.93   | 0.986   | 2.86   | 0.00152               | 12.5   |
|          | 64   | 24.1 ms          | 5.52 ms   | 1.41   | 1.05      | 1.23   | 0.589   | 1.99   | 0.00456               | 7.43   |
|          | 128  | 24 ms            | 5.65 ms   | 0.952  | 0.721     | 0.809  | 0.379   | 1.4    | 0.0017                | 4.31   |
|          | 256  | 23.9 ms          | 5.42 ms   | 0.664  | 0.506     | 0.572  | 0.265   | 0.944  | 0.00114               | 3.48   |
|          | 512  | 23.7 ms          | 5.31 ms   | 0.481  | 0.347     | 0.421  | 0.212   | 0.696  | $3.03 \times 10^{-4}$ | 1.89   |
|          | 1024 | 23.9 ms          | 5.47 ms   | 0.329  | 0.248     | 0.28   | 0.128   | 0.474  | $9.07 \times 10^{-4}$ | 1.31   |
|          | 2048 | 24.1 ms          | 5.6 ms    | 0.233  | 0.173     | 0.197  | 0.095   | 0.33   | $8.12 \times 10^{-4}$ | 1.07   |
|          | 4096 | 24.5 ms          | 5.87 ms   | 0.164  | 0.122     | 0.139  | 0.0687  | 0.234  | $9.51 \times 10^{-5}$ | 0.715  |
|          | 8192 | 24.3 ms          | 5.71 ms   | 0.117  | 0.0879    | 0.0971 | 0.0475  | 0.172  | $1.24 \times 10^{-6}$ | 0.523  |
| 100      | 2    | 25.8 ms          | 5.77 ms   | 99.3   | 0.00396   | 99.3   | 99.3    | 99.3   | 99.3                  | 99.4   |
|          | 4    | 25.6 ms          | 5.84 ms   | 98     | 0.039     | 98     | 98      | 98     | 98                    | 98.3   |
|          | 8    | 25.1 ms          | 5.59 ms   | 62.9   | 21.6      | 68.2   | 52.9    | 76.7   | 0.118                 | 318    |
|          | 16   | 25.2 ms          | 5.61 ms   | 32.6   | 20.2      | 32.9   | 17.3    | 45.6   | 0.214                 | 238    |
|          | 32   | 25.5 ms          | 5.81 ms   | 21.3   | 15.6      | 18.9   | 8.77    | 31     | 0.00838               | 106    |
|          | 64   | 25.5 ms          | 5.88 ms   | 14.9   | 10.7      | 13.3   | 6.45    | 21.3   | 0.0723                | 82.3   |
|          | 128  | 25.1 ms          | 5.78 ms   | 10.1   | 7.74      | 8.59   | 4.08    | 14.3   | 0.00308               | 48.2   |
|          | 256  | 25.3 ms          | 5.96 ms   | 7.23   | 5.49      | 6.13   | 2.91    | 10.1   | 0.0143                | 45.3   |
|          | 512  | 25 ms            | 5.53 ms   | 4.97   | 3.83      | 4.17   | 1.82    | 7.21   | 0.00159               | 26.3   |
|          | 1024 | 25.1 ms          | 5.69 ms   | 3.44   | 2.58      | 2.9    | 1.37    | 4.9    | $4.13 \times 10^{-4}$ | 13.9   |
|          | 2048 | 25.3 ms          | 5.85 ms   | 2.56   | 1.86      | 2.17   | 1.07    | 3.62   | 0.00346               | 10.4   |
|          | 4096 | 24.9 ms          | 5.43 ms   | 1.83   | 1.41      | 1.46   | 0.732   | 2.65   | $7.55 \times 10^{-4}$ | 8.4    |
|          | 8192 | 25.4 ms          | 5.61 ms   | 1.28   | 1.01      | 1.04   | 0.484   | 1.83   | 0.00128               | 5.83   |

Table 12: **Simulation study.** Results for estimator **BayesEst-3-xy**. Mean, standard deviation, median, [0.25, 0.75] quantile, min and max of absolute error.

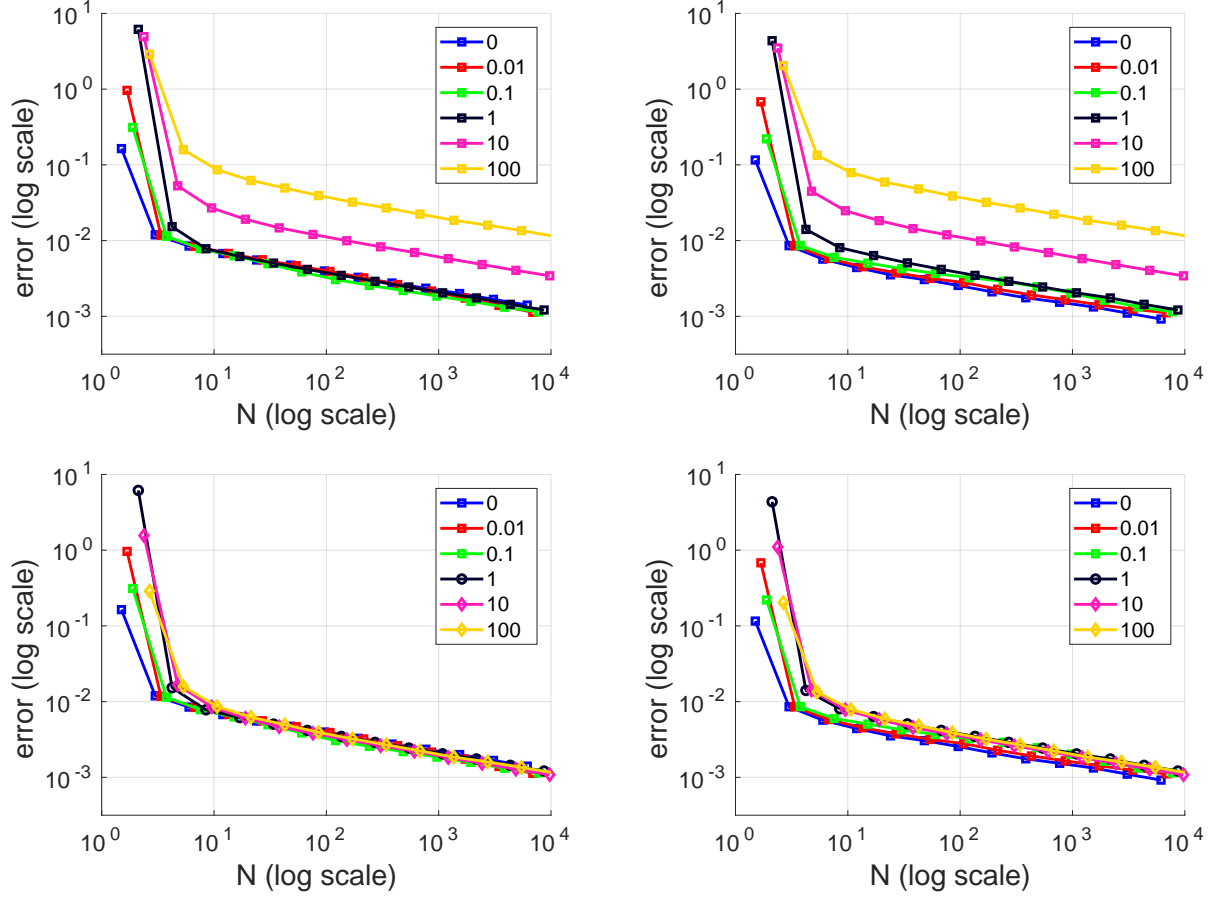

Figure 1: **Simulation study.** Results for estimators jML (left) and mML (right). Top: Error. Bottom: error for  $\kappa \leq 1$  (squares) and relative error for  $\kappa > 1$  (circles).

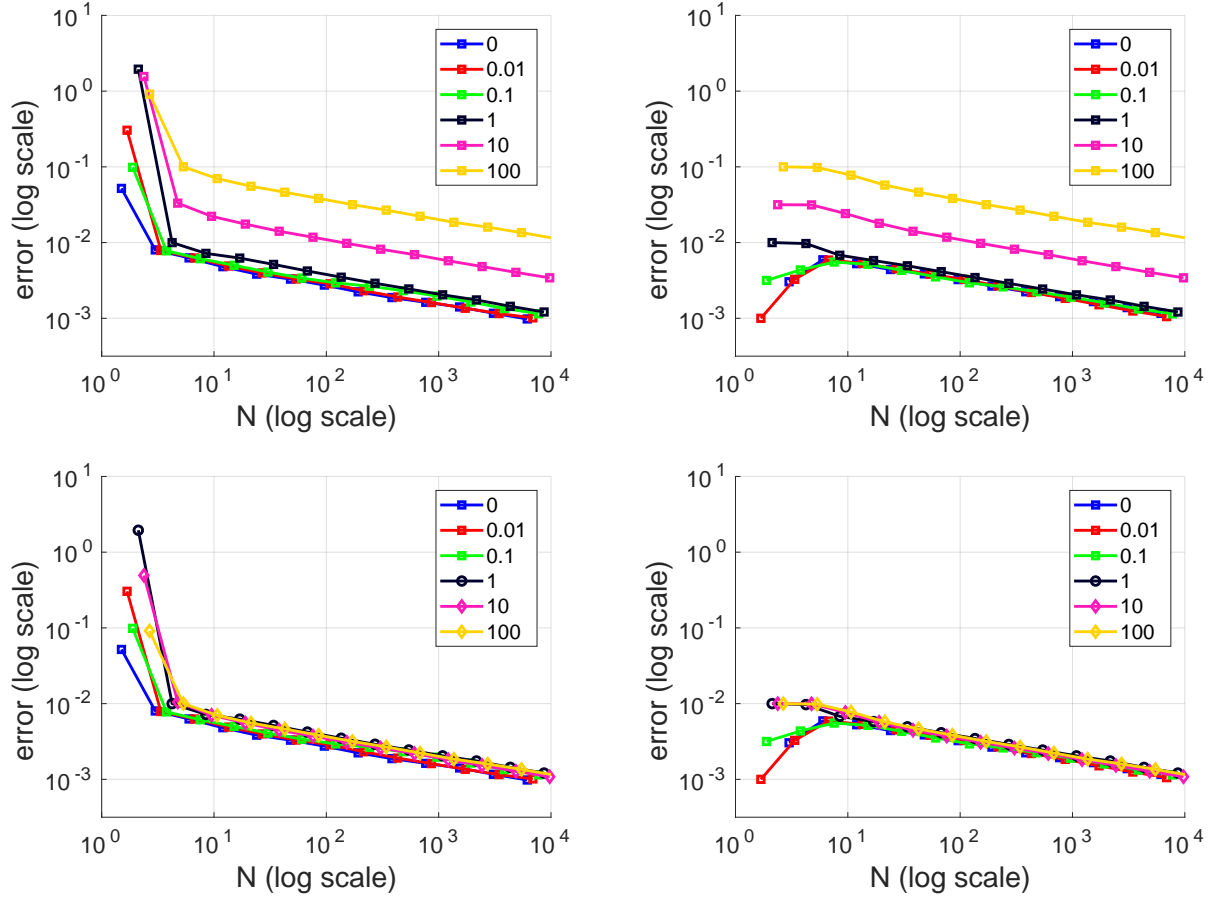

Figure 2: **Simulation study.** Results for estimators BF1 (left) and BF2 (right). Top: Error. Bottom: error for  $\kappa \leq 1$  (squares) and relative error for  $\kappa > 1$  (circles).

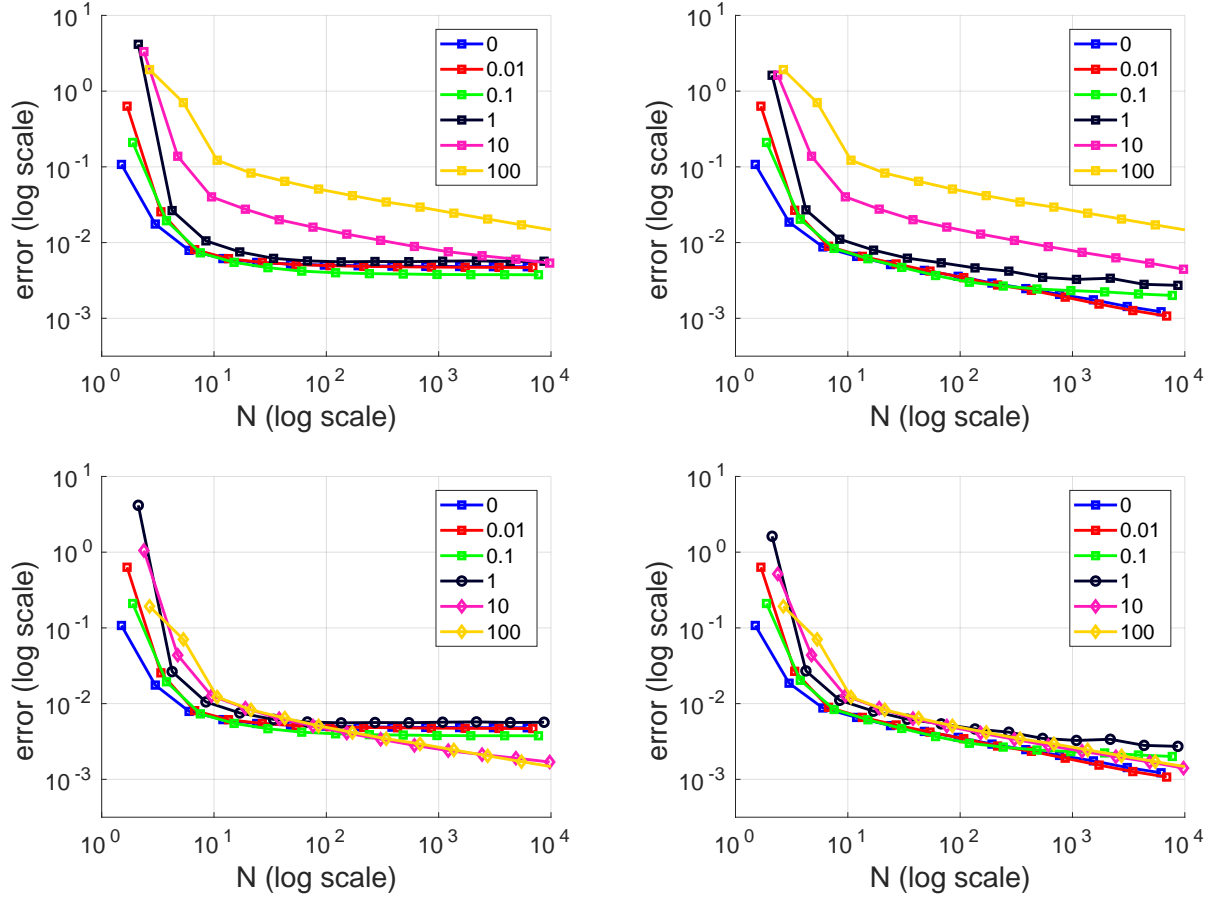

Figure 3: **Simulation study.** Results for estimators `median1` (left) and `median2` (right). Top: Error. Bottom: error for  $\kappa \leq 1$  (squares) and relative error for  $\kappa > 1$  (circles).

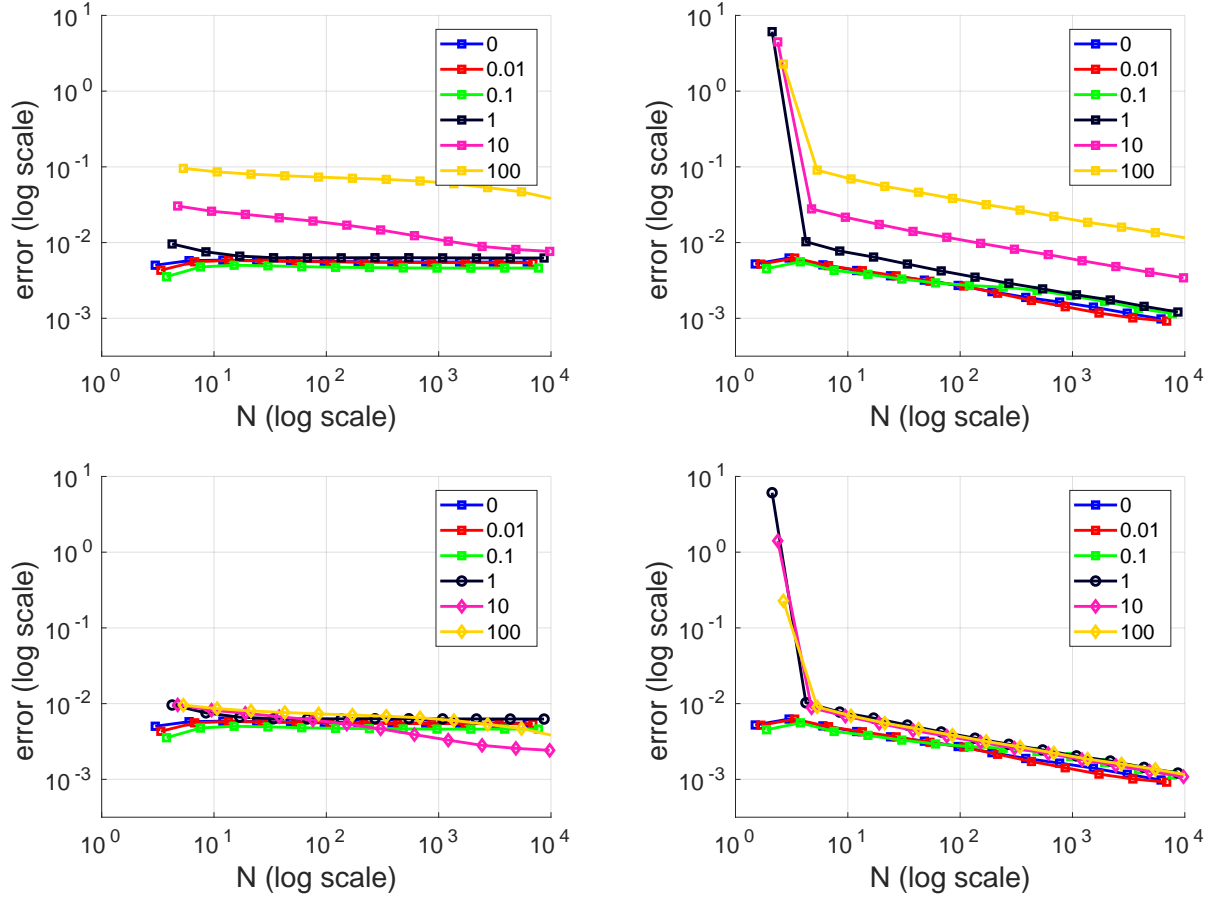

Figure 4: **Simulation study.** Results for estimators `linear` (left) and `MML-2` (right). Top: Error. Bottom: error for  $\kappa \leq 1$  (squares) and relative error for  $\kappa > 1$  (circles).

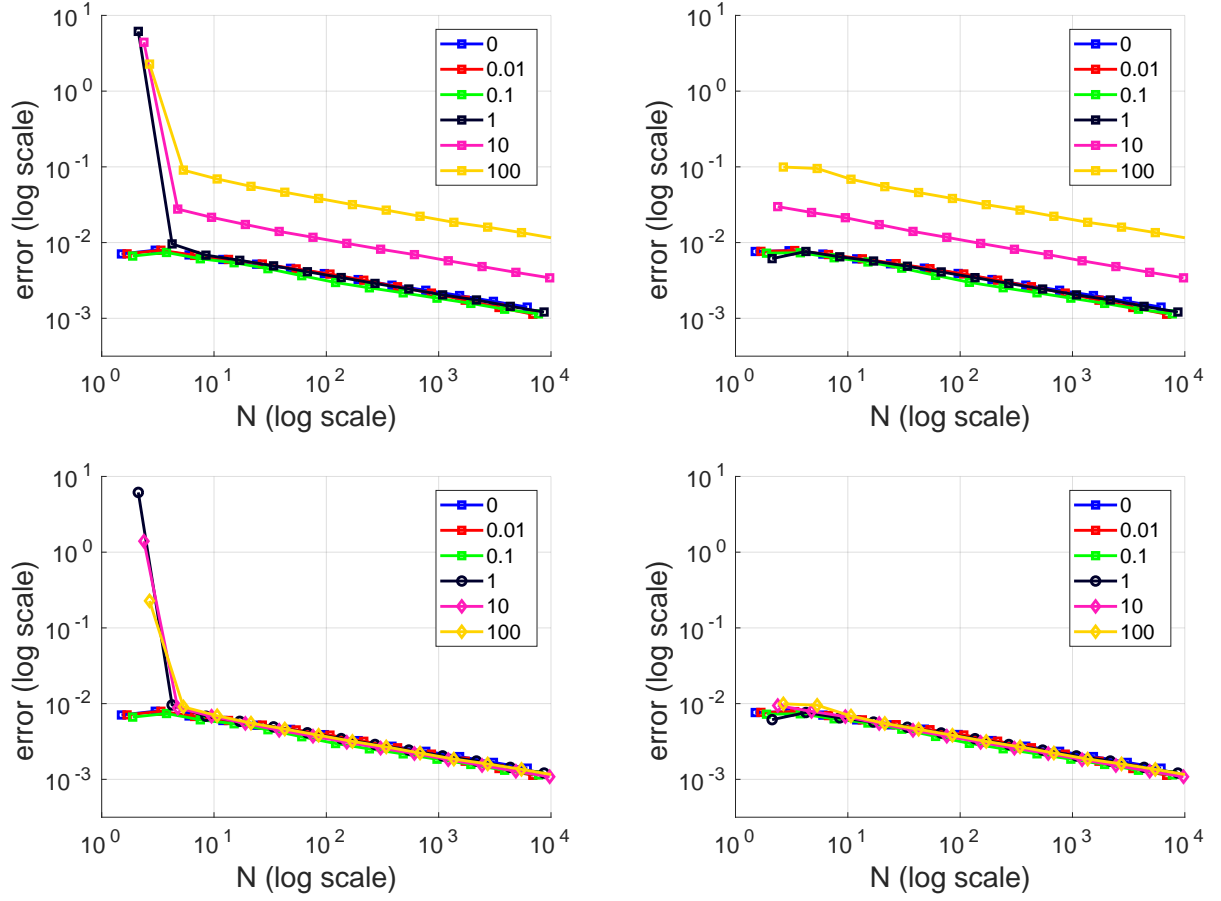

Figure 5: **Simulation study.** Results for estimators MML-3 (left) and BayesEst-2-km (right). Top: Error. Bottom: error for  $\kappa \leq 1$  (squares) and relative error for  $\kappa > 1$  (circles).

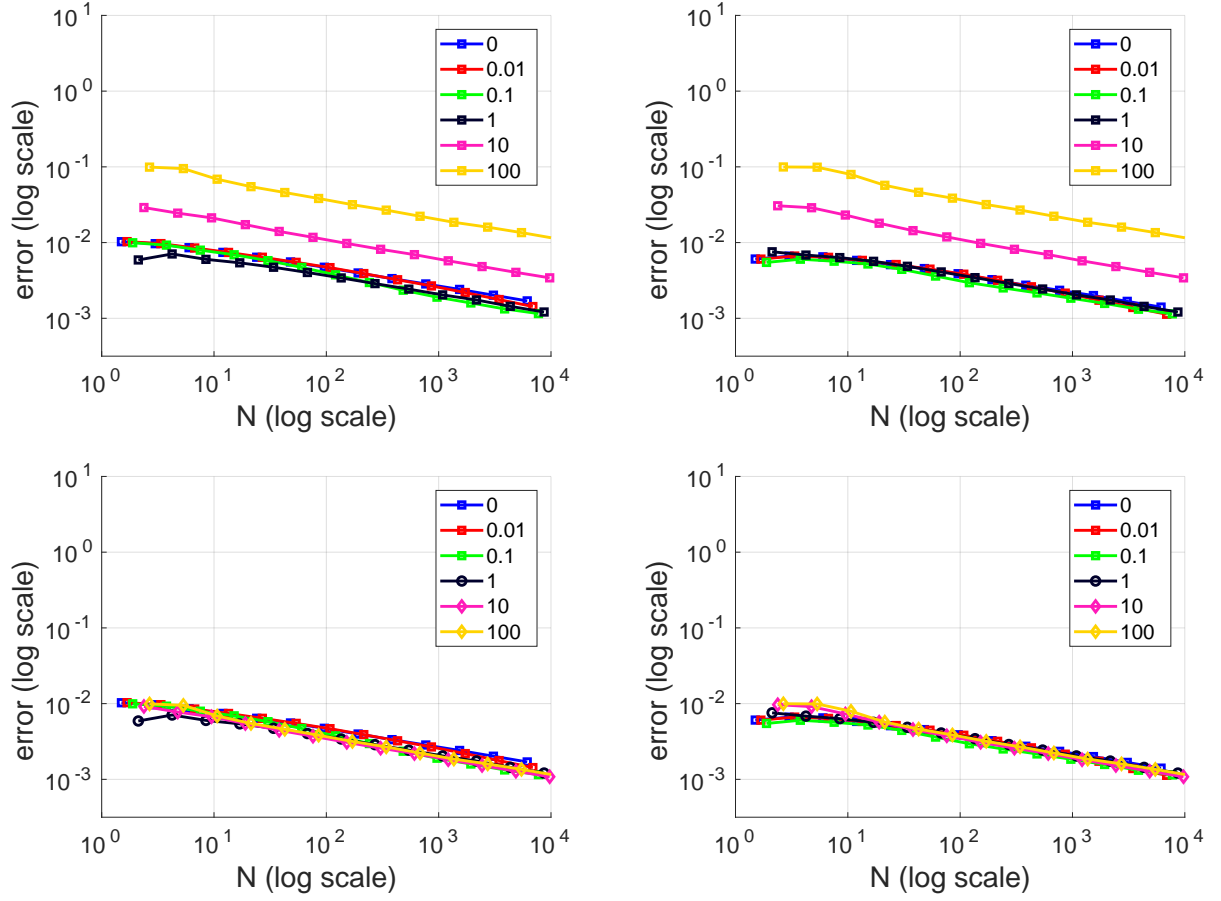

Figure 6: **Simulation study.** Results for estimators BayesEst-3-km (left) and BayesEst-3-xy (right). Top: Error. Bottom: error for  $\kappa \leq 1$  (squares) and relative error for  $\kappa > 1$  (circles).
